# Supplementary material for: Generative assimilation and prediction for weather and climate
Source: arXiv:2503.03038 source file (2025-03-04)
Supplement: Supplementary file 1 [file Supplimentary_Material.tex]

%\documentclass[pdflatex,sn-mathphys-num]{sn-jnl}

%\usepackage{graphicx}%
%\usepackage{multirow}%
%\usepackage{amsmath,amssymb,amsfonts}%
%\usepackage{amsthm}%
%\usepackage{mathrsfs}%
%\usepackage[title]{appendix}%
%\usepackage{xcolor}%
%\usepackage{textcomp}%
%\usepackage{manyfoot}%
%\usepackage{booktabs}%
%\usepackage{algorithm}%
%\usepackage{algorithmicx}%
%\usepackage{algpseudocode}%
%\usepackage{listings}%

%\theoremstyle{thmstyleone}%
%\newtheorem{theorem}{Theorem}%  meant for continuous numbers
%%\newtheorem{theorem}{Theorem}[section]% meant for sectionwise numbers
%% optional argument [theorem] produces theorem numbering sequence instead of independent numbers for Proposition
%\newtheorem{proposition}[theorem]{Proposition}% 
%%\newtheorem{proposition}{Proposition}% to get separate numbers for theorem and proposition etc.

%\theoremstyle{thmstyletwo}%
%\newtheorem{example}{Example}%
%\newtheorem{remark}{Remark}%

%\theoremstyle{thmstylethree}%
%\newtheorem{definition}{Definition}%

%\raggedbottom
%%\unnumbered% uncomment this for unnumbered level heads

\begin{bibunit}

%\begin{document}

\section*{\centering Supplementary information}

\setcounter{figure}{0}

\maketitle

\addtocontents{toc}{\protect\setcounter{tocdepth}{2}}

\tableofcontents
\newpage

\section{Data}\label{Appendix_data_A}

\subsection{Training data}\label{Training_data}

The ERA5 reanalysis dataset, developed by the European Centre for Medium-Range Weather Forecasts (ECMWF), provides comprehensive global reanalysis of weather from 1979 to the present at hourly intervals \cite{hersbach2020era5}. This state-of-the-art reanalysis combines ECMWF's Integrated Forecast System (IFS) cycle 42r1 with an ensemble 4D-Var data assimilation scheme to generate a consistent reconstruction of atmospheric states. ERA5's native spatial resolution of approximately 31 km (0.28125°), providing high-detail information on hundreds of static, surface, and atmospheric variables.

For this study, we utilized the ERA5 version available through the Copernicus Climate Change Service's Climate Data Store (CDS). This dataset has been regridded to a 0.25° equiangular latitude/longitude grid for accessibility and computational efficiency. Additionally, we employ a conservatively regridded 1° grid for specific experimental comparisons with other models and benchmarks.
%Observational data within 12-hour assimilation windows (21–09 UTC and 09–21 UTC) are integrated with previous forecasts to reconstruct a dense and accurate representation of the atmospheric state for each historical date and time. 

Our training dataset comprises ERA5 reanalysis data spanning from 1979-01-01 to 2017-12-31 and includes a selection of variables (SI Table \ref{Appendix_table_variables}) on 13 standard pressure levels, corresponding to those used in the WeatherBench2 benchmark \cite{rasp2024weatherbench}. These pressure levels include: 50, 100, 150, 200, 250, 300, 400, 500, 600, 700, 850, 925, and 1000 hPa. Hourly data were used for training purposes, ensuring high temporal resolution in downstream modeling tasks. This high-fidelity training dataset establishes a robust foundation for atmospheric science research and model benchmarking, combining meteorological accuracy with temporal consistency—essential characteristics for rigorous evaluation of contemporary weather prediction systems and climate models.

\begin{table}[h]
\centering
\caption{Weather variables and levels modeled by GAP. The numbers in parentheses in the column headings are the number of entries in the column. All atmospheric variables are represented at each of the pressure levels.}
\begin{tabular}{lccc}
\toprule
\textbf{Type} & \textbf{Variable name} & \textbf{Short name} & \textbf{ECMWF ID} \\
\midrule
Atmospheric & Geopotential  & z  & 129  \\
Atmospheric          & Specific humidity                   & q                   & 133   \\
Atmospheric          & Temperature                         & t                   & 130      \\
Atmospheric          & U component of wind                 & u                   & 131       \\
Atmospheric          & V component of wind                 & v                   & 132         \\
Single               & 2 metre temperature                 & 2t                  & 167      \\
Single               & 10 metre u wind component           & 10u                 & 165       \\
Single               & 10 metre v wind component           & 10v                 & 166      \\
Single               & Mean sea level pressure             & msl                 & 151          \\
\bottomrule
\end{tabular}
\end{table}\label{Appendix_table_variables}

\subsection{Initial conditions}\label{initial_conditions}
For evaluating GAP's data assimilation performance, we employ initial conditions derived from ECMWF's High-Resolution Forecast (IFS HRES analysis), ECWMF's operational assimilation system that serves as a strong baseline. Operational analyses serve as a reliable reference to assess assimilation quality. Following Lam et al.~\cite{lam2023learning} and Rasp et al.~\cite{rasp2024weatherbench}, we define the initial conditions—specifically, the IFS HRES forecasts at \( t = 0 \)—as ``analysis.''

It is worth noting that this dataset differs slightly from the official analysis product available in the ECMWF archive. The primary distinction lies in the absence of an additional surface data assimilation step that is present in the official product. While this methodological difference has minimal impact on overall evaluation metrics, its effects are most pronounced in the initial time steps post-initialization, particularly for surface temperature variables \cite{price2024probabilistic}. Therefore, interpretation of results at very short lead times warrants careful consideration, though broader evaluation conclusions remain robust.

%Early forecast errors, often transient in nature, tend to dominate evaluation metrics during these periods, rendering them less representative of the overall forecast performance.

\subsection{Operational observation}\label{Operational observation}
\subsubsection{Integrated Global Radiosonde Archive (IGRA)}
The Integrated Global Radiosonde Archive (IGRA) is the largest publicly available collection of quality-controlled radiosonde and pilot balloon observations, providing globally distributed and historical datasets. IGRA is maintained and distributed by the National Centers for Environmental Information (NCEI) under NOAA. The latest version of IGRA was released in 2023 and includes more than 50 million soundings collected from over 2,800 globally distributed stations, including several ship-based stations.
% (Fig.~\ref{ISD_IGRA_view}). 

This dataset spans a wide temporal range, with the earliest records dating back to 1905. Approximately 900 stations worldwide currently contribute daily updates to the archive, ensuring its relevance for both historical and near-real-time atmospheric studies. Each sounding provides vertical profiles of atmospheric variables, which may include temperature, humidity, wind speed and direction, as well as the height of each observation. Heights are typically reported in terms of pressure and/or geopotential height, depending on the station and time of observation.

IGRA’s extensive temporal and spatial coverage, coupled with its rigorous quality control measures, makes it a critical resource for atmospheric research and climate studies. The archive’s unique combination of historical depth and contemporary updates enables detailed investigations into long-term atmospheric trends and variability.

\subsubsection{Global Hourly Integrated Surface Database (ISD)}
The Integrated Surface Database (ISD) is a comprehensive global archive of hourly and synoptic surface observations, compiled from a wide range of sources. Maintained by NOAA's National Centers for Environmental Information (NCEI), ISD integrates data from over 100 original sources, ensuring the preservation and accessibility of valuable historical surface weather observations.

ISD contains a wide array of meteorological parameters observed at individual stations, including wind speed and direction, wind gusts, temperature, dew point, cloud cover, sea level pressure, altimeter settings, station pressure, present weather conditions, visibility, precipitation amounts over various time intervals, and snow depth. The database also includes other site-specific variables depending on the observing station. With its extensive spatial and temporal coverage, ISD serves as a vital resource for atmospheric and climate research. Its integration of historical and modern observations supports diverse applications, including reanalysis, model validation, and long-term trend analysis. ISD’s commitment to data quality and consistency ensures its ongoing utility for global scientific studies.

% \begin{figure}[h]
% \centering
% \centerline{\includegraphics[width=\linewidth]{suppli_fig/ISD_IGRA_view.jpg}}
% \caption{Surface measurements and sounding stations distribution of ISD (left) and IGRA (right)}\label{ISD_IGRA_view}
% \end{figure}

\subsection{Data preprocessing}\label{SI_section1_data_preprocessing}

The ISD and IGRA datasets contain missing values (NaNs) and unreasonable entries caused by measurement errors. To prevent erroneous inferences in GAP, this data was preprocessed according to specific criteria prior to analysis.

For near-surface wind components (\(u\) and \(v\)), preprocessing involved filtering out missing values and addressing anomalies. Anomalous stations, even those with recorded data, were masked by setting the corresponding mask values to zero (\(\text{mask} = 0\)). Additionally, integer grid cells without stations within a 0.25° longitude radius were also masked (\(\text{mask} = 0\)). Despite these preprocessing efforts, significant discrepancies remained between the near-surface \(u\) and \(v\) components and the ERA5 dataset. This indicates that the applied masking strategies were insufficient to fully resolve the differences.

For surface air temperature, surface pressure, and radiosonde data, a simplified preprocessing approach was adopted. Specifically, only missing values were filtered out, without employing the additional masking procedures used for \(u\) and \(v\). This approach emphasizes data integrity by focusing on retaining reliable and valid measurements while minimizing the complexity of preprocessing.

All grid based model data were regridded using first-order conservative regridding following Rasp et al. \cite{kochkov2024neural, rasp2024weatherbench}, i.e., with weights proportional to the area of overlap between grid cells on the original and desired grids.

\clearpage

\section{Model specification}\label{Appendix_method_B}

The goal of GAP is to model the joint probability distribution:

\begin{equation*}
p(\mathbf{X}_{0:t}|\Theta, \mathbf{O}_{t_0:0}),
\label{eq:joint_distribution}
\end{equation*}

where $\mathbf{X}_{0:t}$ represents the sequence of atmospheric states from $t=0$ to $t$, $\mathbf{O}_{t_0:0}$ denotes the observational data from time $t_0$ to $0$, and $\Theta$ represents the climatological prior parameters. This joint distribution can be split into two components:

\begin{equation*}
p(\mathbf{X}_{0:t}|\Theta, \mathbf{O}_{t_0:0}) = 
p(\mathbf{X}_0|\Theta, \mathbf{O}_{t_0:0}) \cdot 
p(\mathbf{X}_{1:t}|\Theta, \mathbf{X}_0).
\label{eq:assimilation_prediction_split}
\end{equation*}

In the assimilation phase, the goal is to estimate the initial state $\mathbf{X}_0$ conditioned on the observational data $\mathbf{O}_{t_0:0}$ and the climatological prior $p(\mathbf{X}_{\bar{t}}|\Theta)$. Using Bayes' theorem:

\begin{equation*}
p(\mathbf{X}_0|\Theta, \mathbf{O}_{t_0:0}) = 
\frac{p(\mathbf{O}_{t_0:0}|\mathbf{X}_0, \Theta) \cdot p(\mathbf{X}_0|\Theta)}{p(\mathbf{O}_{t_0:0}|\Theta)}.
\label{eq:bayes_theorem}
\end{equation*}

Here $p(\mathbf{X}_0|\Theta)$ is the climatological prior. $p(\mathbf{O}_{t_0:0}|\mathbf{X}_0, \Theta)$ is the likelihood of observations given the state $\mathbf{X}_0$. $p(\mathbf{O}_{t_0:0}|\Theta)$ is a normalization factor.

Observations at each time step are conditionally independent given the corresponding state. The observational data $\mathbf{O}_{t_0:0}$ consists of a sequence of observations, and its likelihood can be decomposed as:

\begin{equation*}
p(\mathbf{O}_{t_0:0}|\mathbf{X}_0, \Theta) = \prod_{i=t_0}^0 p(\mathbf{O}_i|\mathbf{X}_i, \Theta).
\label{eq:observation_likelihood}
\end{equation*}

Here, $p(\mathbf{O}_i|\mathbf{X}_i, \Theta)$ represents the likelihood of the observation at time $i$ given the state $\mathbf{X}_i$.

We make a second-order Markov approximation. The state evolution can be written as:

\begin{equation*}
p(\mathbf{X}_{t_0:0}|\Theta) = p(\mathbf{X}_{t_0}|\Theta) \prod_{i=t_0}^1 p(\mathbf{X}_i|\mathbf{X}_{i-1}).
\label{eq:state_evolution}
\end{equation*}

Combining the likelihood of observations and the dynamical evolution of states, the assimilation phase can be expressed as:

\begin{equation*}
p(\mathbf{X}_0|\Theta, \mathbf{O}_{t_0:0}) = 
p(\mathbf{X}_{\bar{t}}|\Theta) 
\prod_{i=t_0}^0 \frac{p(\mathbf{O}_i|\mathbf{X}_i, \Theta) \cdot p(\mathbf{X}_i|\mathbf{X}_{i-1})}{p(\mathbf{O}_i|\Theta)}.
\label{eq:assimilation_phase}
\end{equation*}

In the prediction phase, the goal is to estimate the future states $\mathbf{X}_{1:t}$ based on the initial state $\mathbf{X}_0$. Under the Markov assumption, the future states can be factorized as:

\begin{equation*}
p(\mathbf{X}_{1:t}|\Theta, \mathbf{X}_0) = \prod_{i=1}^t p(\mathbf{X}_i|\mathbf{X}_{i-1}).
\label{eq:prediction_phase}
\end{equation*}

The dynamical evolution term $p(\mathbf{X}_i|\mathbf{X}_{i-1})$ can be defined using either physical models or data-driven machine learning models. In GAP, this is implemented using a diffusion model to account for stochastic variability and systematic bias correction.

Combining the assimilation and prediction phases, the complete joint distribution is:

\begin{equation*}
p(\mathbf{X}_{0:t}|\Theta, \mathbf{O}_{t_0:0}) = 
p(\mathbf{X}_{\bar{t}}|\Theta) 
\prod_{i=t_0}^0 \frac{p(\mathbf{O}_i|\mathbf{X}_i, \Theta) \cdot p(\mathbf{X}_i|\mathbf{X}_{i-1})}{p(\mathbf{O}_i|\Theta)} 
\prod_{i=1}^t p(\mathbf{X}_i|\mathbf{X}_{i-1}).
\label{eq:complete_formula}
\end{equation*}

The foundation of GAP lies in the use of probabilistic diffusion models to parameterize target distributions. These models, acting as generative frameworks for data, operate through a Markov chain process. Commencing with a stochastic draw from an initial noise distribution—often an isotropic multivariate Gaussian—the model undergoes iterative transformations and denoising until it converges to a representation resembling a random sample from the actual data distribution\cite{song2019generative, song2020sliced, sohl2015deep, kingma2021variational}. These iterative steps are governed by diffusion time schedule.

The denoising procedure hinges upon the instantiation of a diffusion time–dependent score function, derived from the Jacobian of the log likelihood of the data at a specific diffusion time. Frequently, these score functions are realized through deep learning architectures whose parameters are honed through training data.

The score function operates simultaneously on both the noisy sample and the diffusion time parameter, creating a model that effectively encapsulates the unconditional distribution of the training data\cite{song2020score}. For GAP, we employ the vanilla U-Net architecture\cite{ronneberger2015u} as our score function implementation, selected for its proven efficacy across diverse generative modeling tasks\cite{song2020score, meng2021sdedit} and its ability to capture multi-scale atmospheric patterns.

Our key innovation is to model $p(X^t)$ or the gradient of distribution of ERA5 with a learned neural network-based diffusion model\cite{karras2022elucidating, sohl2015deep, song2020sliced}, which allows us to draw samples from it. GAP can sample $X^t$ directly, with a fake generation similar to weather state in ERA5. Our approach is to sample conditionally $Z^t$ with respect to weather state $X^{t-1}$, partial observations or external forcing using various guiding techniques.

%We broadly follow the diffusion framework presented in Lugmayr et al.\cite{lugmayr2022repaint}.

%\clearpage

%\section{Sampling techniques}\label{Appendix_method_C}

Ideally, an unconditional diffusion based generative method should provide exact samples for a broad range of conditional distributions without requiring task specific training. To help with this expense, a separate line of work uses heuristic approximations that directly operate on unconditional diffusion models: once an unconditional model $p_{\Theta}(x)$ is trained, it can be flexibly combined with various conditioning criteria to generate customized outputs \cite{song2020score, daras2024survey}.

Gupta et al. \cite{gupta2024diffusion} shows that there are instances of the posterior sampling problem for which every algorithm takes superpolynomial time, even though unconditional sampling is provably fast. Hence, diffusion models excel at performing unconditional sampling but are hard to use as priors for solving inverse problems because of the time dependence in the measurements matching term. Since the very introduction of diffusion models, there has been a plethora of methods proposed to use them to solve inverse problems without retraining. Here we introduce some guidance techniques used in GAP.

\subsection{Diffusion settings}\label{diffusion_settings}

\subsubsection{Sampling process}

The sampling process begins by drawing an initial sample $Z_0^t$ from a Gaussian noise distribution at a high initial noise level $\sigma_0$. After $N$ transformation steps, we obtain $Z_N^t := Z^t$, a sample from the target distribution at noise level $\sigma_N = 0$. This transformation is performed by applying an ordinary differential equation (ODE) solver to the probability flow ODE, as described by Karras et al.\cite{karras2022elucidating}, and Song et al.\cite{song2020sliced}. Each step of this solver is denoted by $r_\theta$, and is represented mathematically as:

\begin{equation*}
Z_{i+1}^t = r_\theta(Z_i^t, \sigma_{i+1}, \sigma_i),
\end{equation*}

where the solver transitions the sample from noise level $\sigma_i$ to the subsequent lower noise level $\sigma_{i+1}$ unconditionally.

To solve this ODE, we employ the DDPM algorithm\cite{lugmayr2022repaint, song2020score}, augmented with stochastic churn and noise inflation techniques as proposed by Karras et al.\cite{karras2022elucidating}. These enhancements incorporate additional stochasticity into the sampling process by leveraging $p_{\text{noise}}$ (detailed in Section D.2).

Each solver step $r_\theta$ leverages a learned denoiser $D_\theta$ parameterized by $\theta$. The specific details of the denoiser are elaborated in Section D.3. For our implementation, we use $N = 160$ solver steps for both assimilation and prediction phase. Given that the solver operates at second-order accuracy, each step $r_\theta$ necessitates two evaluations of the denoiser $D_\theta$, except for the final step, which requires only one evaluation. Consequently, the total number of denoiser evaluations for the sampling process is given by $N - 1$. For further details, including a comprehensive list of sampling hyperparameters, please refer to SI Section \ref{training_details}.

\subsubsection{Noise schedule}

At the core of a diffusion model lies a fundamental process involving the sequential addition and removal of noise. This noise is sampled from a specific distribution, denoted as $p_{\text{noise}}(\cdot|\sigma)$, where $\sigma$ represents the noise level that parametrizes the distribution. The choice of this distribution significantly influences the behavior and theoretical foundation of the diffusion model.

A common approach is to define $p_{\text{noise}}$ as an independent and identically distributed Gaussian noise model. This choice was popularized in the seminal work of Ho et al.\cite{ho2020denoising}, which demonstrated the efficacy of diffusion models in producing high-quality image samples. Specifically, the Gaussian white noise assumption simplifies the theoretical analysis and practical implementation of these models, allowing researchers to leverage established probabilistic frameworks and sampling techniques. In the GAP, we broadly use the common noise schedule above for smoothly adpting various guiding techniques.

%The standard theory surrounding diffusion models has been primarily developed under the assumption of Gaussian noise. This includes methodologies for training such models, understanding their convergence properties, and analyzing their expressive power. While alternative noise distributions could theoretically be employed, the Gaussian white noise assumption remains dominant due to its mathematical tractability and empirical success in image synthesis tasks. 

\subsubsection{Denoiser architecture}

The diffusion sampling process is built upon iterative solver steps denoted as $r_\theta$. Each solver step incorporates a denoiser $D_\theta$ as an integral component of its computation. In GAP, the denoiser, $D_\theta$, is parameterized using a U-Net architecture, as described in Ronneberger et al. \cite{ronneberger2015u}. This parameterization represents $D_\theta$ as a preconditioned form of a neural network function $f_\theta$. Key adaptations were made to align with the requirements of the diffusion model:

\begin{itemize}
    \item \textbf{Encoder-Decoder Structure:} The encoder compresses the input features through a sequence of downsampling and convolutional operations, while the decoder restores the resolution through upsampling and transposed convolutions. Skip connections are employed between corresponding layers of the encoder and decoder to preserve high-resolution details.
    \item \textbf{Normalization of Inputs:} Inputs to the encoder, corresponding to noise-corrupted versions of the target from the previous two timesteps, are normalized to zero mean and unit variance to ensure consistency across varying noise levels.
    \item \textbf{Preconditioning with Noise Scaling:} The preconditioning functions $c_\text{in}$ and $c_\text{noise}$ modulate the input features and noise-level embeddings, respectively, ensuring that the model efficiently handles different noise scales.
\end{itemize}

This parameterization and architectural choice ensure robust denoising capabilities across a wide range of noise levels, a critical requirement for accurate image synthesis in diffusion models.

\subsubsection{Training details}\label{training_details}

During training, we apply the denoiser $D_\theta$ to a noise-corrupted atmospheric state $X^t$ by adding noise $\epsilon \sim p_{\text{noise}}(\cdot|\sigma)$ at noise level $\sigma$:

\begin{equation*}
Y^t = D_\theta(X^t + \epsilon; \sigma)
\end{equation*}

We optimize the denoiser to predict the original noise-free state by minimizing the weighted mean-squared-error:

\begin{equation*}
\mathcal{L} = \sum\mathbb{E}{\sigma, \epsilon} \left[\lambda(\sigma) \sum_{i \in G} \sum_{j \in J}(Y^t_{i,j} - X^t_{i,j})^2\right]
\end{equation*}

where $j$ indexes variables and pressure levels (e.g., $J = {z{1000}, z_{850}, \ldots, 2T, \text{mslp}}$), $i$ indexes latitude-longitude coordinates, $\lambda(\sigma)$ is the noise-level-dependent weighting function from Karras et al \cite{karras2022elucidating}.

We sample noise levels by drawing $u \sim U[0, 1]$ and applying a transformation to obtain a log-normally distributed $\sigma$. During training, we use the same noise schedule parameter $\rho$ as at sampling time, but with a slightly wider range for $[\sigma_{\min}, \sigma_{\max}]$ to enhance model robustness.

%We implemented all methods on the NVIDIA Geforce 4090 24GB GPU using CUDA version 12.3. 
Hyperparameter configurations for diffusion models are often adopted from the ho et al.\cite{ho2022classifier}. Some specific hyperparameters of the model are presented in the following table.~\ref{tab:hyperparameter}. We conduct training using the Adam optimizer with a learning rate of $1e^{-4}$, batch size of 4, and continue for over 1000 epochs.

\begin{table}[htbp]
  \centering
  \caption{Hyperparameters of the diffusion model}
  \label{tab:hyperparameter}
  \begin{tabular}{lc}
    \toprule
    \textbf{Hyperparameter} & \textbf{Setting} \\
    \midrule
    Learning Rate & $10^{-4}$ \\
    Optimizer & Adam \\
    Batch Size & 4 \\
    Activation Function & ReLU \\
    Channel & 256 \\
    Epochs & 1000 \\
    \bottomrule
  \end{tabular}
\end{table}

\subsubsection{Experiment time}\label{Experiment_time}

Table~\ref{tab:Experiment_time} presents the inference time of the GAP model across different tasks. The experiments were conducted using a single ensemble member, and all tests were performed on a standard Nvidia RTX 4090 Graphics Processing Unit (GPU). The denoising process consists of 80 steps, while the initial noise level for SDEdit is set at 40 steps. Each ensemble member requires 7.84 GB of GPU memory, allowing a single Nvidia RTX 4090 to run up to 3 ensemble members in parallel.

\begin{table}[htbp]
  \centering
  \caption{Inference time of GAP across different tasks}
  \label{tab:Experiment_time}
  \begin{tabular}{lc}
    \toprule
    \textbf{Experiment type} & \textbf{Time} \\
    \midrule
    Random generation & 2.4s \\
    Assimilation (3-day time window) & 2min 17.1s \\
    15-d forecast & 31.5s \\
    3-month prediction & 3min 13.4s \\
    40-year simulation & 8h 31min 21.0s \\
    \bottomrule
  \end{tabular}
\end{table}

\subsubsection{Random sampling}\label{DDIM}

In this section, we provide the base random inference method of GAP. We include just enough details to explain our proposed approach and recommend readers consult the original papers for complete derivations and explanations \cite{song2020denoising}.

Denote $\mathbf{X}_0$ as a random vector representing atmospheric gridded state (vectorized). Denoising Diffusion Implicit Models (DDIM) aim to recover the distribution of $\mathbf{X}0$ through a set of intermediate variables, $\mathbf{X}{1:T}$, which are progressively corrupted versions of $\mathbf{X}_0$. The DDIM framework consists of two main processes. The first process is forward diffusion process: defines how $\mathbf{X}_0$ is corrupted into $\mathbf{X}_T$. The other is reverse denoising Process: governs how to recover $\mathbf{X}_0$ from $\mathbf{X}_T$ based on the forward process.

The forward diffusion process in DDIMs follows that of Denoising Diffusion Probabilistic Models (DDPMs)\cite{sohl2015deep, ho2020denoising}, which is a Markov process that progressively adds Gaussian noise to the intermediate variables. Mathematically, this process is expressed as:

\begin{equation*}
q(\mathbf{X}t | \mathbf{X}{t-1}) = \mathcal{N}(\mathbf{X}t; \sqrt{1-\beta_t} \mathbf{X}{t-1}, \beta_t \mathbf{I}),
\end{equation*}

where $\beta_t \in (0, 1)$ represents the noise schedule at timestep $t$.

The reverse process is parameterized by a neural network $p_\theta$ designed to predict the denoised intermediate variables:

\begin{equation*}
p_\theta(\mathbf{X}{t-1} | \mathbf{X}t) = \mathcal{N}(\mathbf{X}{t-1}; \mu\theta(\mathbf{X}t, t), \Sigma\theta(\mathbf{X}_t, t)).
\end{equation*}

DDIMs modify this framework by introducing a non-Markovian reverse process that preserves the marginal distributions of DDPMs while allowing deterministic sampling paths. For further details, refer to Song et al.\cite{song2020denoising}.

\begin{equation*}
q(\mathbf{X}_{1:T}|\mathbf{X}0) = \prod{t=1}^{T} q(\mathbf{X}t|\mathbf{X}{t-1}),
\end{equation*}

\begin{equation*}
q(\mathbf{X}t|\mathbf{X}{t-1}) = \mathcal{N}(\mathbf{X}t; \sqrt{\alpha_t}\mathbf{X}{t-1}, \beta_t\mathbf{I}),
\end{equation*}

where $\alpha_{1:T}$ and $\beta_{1:T}$ define the scaling and variance schedule with $\alpha_t = 1 - \beta_t$. It can be easily shown that, with an appropriate scaling and variance schedule and a sufficiently large $T$, $\mathbf{X}_T$ approaches the standard Gaussian distribution.

For the reverse diffusion process, DDIMs introduce another distribution $q_\sigma$, called the inference distribution, that has a matching conditional distribution of each individual intermediate variable to $q$. Specifically,

\begin{equation*}
q_\sigma(\mathbf{X}{1:T}|\mathbf{X}0) = q\sigma(\mathbf{X}T|\mathbf{X}0) \prod{t=T}^{2} q\sigma(\mathbf{X}{t-1}|\mathbf{X}_t, \mathbf{X}_0),
\end{equation*}

\begin{equation*}
q_\sigma(\mathbf{X}_T|\mathbf{X}_0) = \mathcal{N}(\mathbf{X}_T; \sqrt{\bar{\alpha}_T}\mathbf{X}_0, (1 - \bar{\alpha}_T)\mathbf{I}),
\end{equation*}

\begin{equation*}
q_\sigma(\mathbf{X}_{t-1}|\mathbf{X}_t, \mathbf{X}0) = \mathcal{N}(\mathbf{X}{t-1}; \mu_t, \sigma_t^2\mathbf{I}),
\end{equation*}

where $\bar{\alpha} = \prod_{i=1}^{t}\alpha_i$ and $\sigma_t^2$ is a free hyperparameter, and

\begin{equation*}
\mu_t = \sqrt{\alpha_{t-1}}\mathbf{X}0 + \sqrt{1 - \bar{\alpha}{t-1} - \sigma_t^2} \frac{\mathbf{X}_t - \sqrt{\alpha_t}\mathbf{X}_0}{\sqrt{1 - \alpha_t}}.
\end{equation*}

It can be shown that as long as $\sigma_t^2 \in [0, 1 - \bar{\alpha}t]$, $\forall t$. $q\sigma$ and $q$ have matching distributions: $q_\sigma(\mathbf{X}_t|\mathbf{X}_0) = q(\mathbf{X}_t|\mathbf{X}_0)$, $\forall t$.

The denoising process is derived from $q_\sigma$ by replacing $\mathbf{X}_0$ with an estimated value of $\mathbf{X}_0$, i.e.,

\begin{equation*}
p_\theta(\mathbf{X}_T) = \mathcal{N}(\mathbf{X}_T; 0, \mathbf{I})
\end{equation*}

\begin{equation*}
p_\theta(\mathbf{X}{t-1}|\mathbf{X}t) = q\sigma(\mathbf{X}{t-1}|\mathbf{X}_t, \hat{\mathbf{X}}_0^{(t)}),
\end{equation*}

where $\hat{\mathbf{X}}_0^{(t)}$ is produced by a (reparameterized) neural network that predicts $\mathbf{X}_0$ from $\mathbf{X}_t$ by minimizing the mean squared error.

Equation 5 provides a way of estimating the final generation as a deterministic function of \(\tilde{\mathbf{X}}_t\). In particular, \(f_\theta^{(t)}(\tilde{\mathbf{X}}_t)\) is generated by feeding to the inference network once, and thus can be regarded as a compute-efficient approximation of the final generation. We will refer to it as one-step generation. As we will show, one-step generation is central to our assimilation guiding algorithm because it permits direct control over the final generation through the intermediate variables.

\subsection{Forecasting model}\label{Forecasting_model}

Our study adopts a data-driven forecast model called \textbf{ConvCast} as the physical transient backbone. ConvCast is a deep learning model specifically designed to predict weather conditions 6 hours ahead. The model architecture adopts the ConvNeXt design \cite{liu2022convnet} and incorporates a UNet-like structure to enable effective feature extraction and representation. The primary objective of ConvCast is to balance lightweight design with high computational efficiency, allowing the model to handle large datasets effectively through a purely convolutional approach.

This purely convolutional design integrates several innovative components to enhance performance:

\begin{itemize}
    \item \textbf{Layer Normalization:} Supports both channel-first and channel-last data formats, ensuring adaptability to diverse input structures.
    \item \textbf{ConvNeXt Blocks:} Embedded within a UNet-like structure, these blocks enhance spatial-temporal pattern recognition.
    \item \textbf{Depthwise Convolutions:} Improve computational efficiency by reducing the number of parameters while maintaining high representational power.
    \item \textbf{Upsampling and Downsampling Modules:} Enable multi-scale feature processing, which is vital for accurate predictions across various spatial resolutions.
\end{itemize}

This architecture enables ConvCast to efficiently process and analyze large meteorological datasets, delivering high performance in forecasting tasks while maintaining computational efficiency.

ConvCast was rigorously trained on 39-year ERA5 reanalysis data (1979-2017, same as GAP) with a spatial resolution of 1 degree. The training process was designed to optimize the model for 6-hour weather condition predictions and included the following components:

\begin{itemize}
    \item \textbf{Loss Function:} Weighted mean squared error was employed as the primary loss function. The weighted component is same as GraphCast \cite{lam2023learning}.
    \item \textbf{Learning Rate Schedule:} An initial learning rate of 0.001 was used, gradually reduced to zero following a cosine annealing schedule. This approach ensures smooth convergence during training.
    \item \textbf{Scheduled DropPath:} A drop ratio of 0.2 was implemented to combat overfitting and enhance model robustness by introducing stochasticity during training.
\end{itemize}

The combination of these strategies resulted in a robust and efficient model capable of delivering accurate 6-hour weather forecasts while maintaining computational efficiency. This balance makes ConvCast suitable for both research and operational forecasting tasks.

%\subsection{Combine techniques across temporal scales}\label{Appendix_B14

\subsection{Inpainting}\label{inpainting_SI}

Inpainting leverages pre-trained diffusion models to generate high-fidelity samples that are faithful to observations, and uncertainty-aware. This methodology combines a learned climatology prior with sparse station observations to infer the posterior probability distribution of the target variable. The key innovation lies in applying observations to guide the pre-trained diffusion model's generation process, requiring no extra training and accommodating arbitrary observation layouts (SI Fig.~\ref{fig_inpainting_SDE}).

The pre-trained diffusion model sequentially applies the reverse process which systematically transforms the prior distribution $p(\mathbf{X}_T)$ into the target distribution $p(\mathbf{X}_0)$. For grid points with observations within a pre-selected time window $\Omega$, the values of $\mathbf{X}_{t}$ are replaced with noisified observations sampled from $p(\mathbf{X}_{t} \odot \mathbf{m} | \mathbf{X}_{0} \odot \mathbf{m})$, where $\mathbf{m}$ is a binary mask representing observed regions.

We now provide a step-by-step derivation of the observational likelihood gradient $\nabla_{\mathbf{x}\tau} \log p(\mathbf{O}|\mathbf{x}\tau)$, which governs how observations influence the diffusion process.

Given our one-step approximation assumptions:

\begin{equation*}
\mathbf{O} \sim \mathcal{N}(\mathbf{O}; \Omega(\mathbf{X}), \mathbf{\Sigma}\mathbf{o})
\end{equation*}

\begin{equation*}
\mathbf{X} \sim \mathcal{N}(\mathbf{X}; F\tau(\mathbf{x}\tau), \mathbf{\Sigma}\mathbf{\tau})
\end{equation*}

By exploiting the conditional independence of observations $\mathbf{O}$ and diffusion state $\mathbf{x}\tau$ given the atmospheric state $\mathbf{X}$:

\begin{equation*}
p(\mathbf{O}, \mathbf{x}\tau|\mathbf{X}) = p(\mathbf{O}|\mathbf{X})p(\mathbf{x}_\tau|\mathbf{X})
\end{equation*}

We marginalize over $\mathbf{X}$ to obtain the conditional probability $p(\mathbf{O}|\mathbf{x}\tau)$:

\begin{equation*}
p(\mathbf{O}|\mathbf{x}\tau) = \int p(\mathbf{O}|\mathbf{X})p(\mathbf{X}|\mathbf{x}\tau)d\mathbf{X} = \mathcal{N}(\mathbf{O}; \Omega(F\tau(\mathbf{x}\tau)), \mathbf{\Sigma}\mathbf{o} + \nabla\Omega \cdot \mathbf{\Sigma}_\tau \cdot \nabla\Omega^\top)
\end{equation*}

Taking the logarithm yields:

\begin{equation*}
\log p(\mathbf{O}|\mathbf{x}\tau) = -\frac{1}{2}(\mathbf{O} - \Omega(F\tau(\mathbf{x}\tau)))^\top
(\mathbf{\Sigma}\mathbf{o} + \nabla\Omega \cdot \mathbf{\Sigma}\tau \cdot \nabla\Omega^\top)^{-1}
(\mathbf{O} - \Omega(F\tau(\mathbf{x}_\tau))) + C
\end{equation*}

Finally, taking the gradient with respect to $\mathbf{x}\tau$ and applying the chain rule:

\begin{equation*}
\nabla{\mathbf{x}\tau} \log p(\mathbf{O}|\mathbf{x}\tau) = (\nabla F_\tau)^\top \cdot (\nabla \Omega)^\top \cdot (\mathbf{\Sigma}\mathbf{o} + \nabla \Omega \cdot \mathbf{\Sigma}\tau \cdot \nabla \Omega^\top)^{-1} \cdot (\mathbf{O} - \Omega(F_\tau(\mathbf{x}_\tau)))
\end{equation*}

This gradient provides the mechanism by which observational information guides the diffusion process, enabling physically consistent atmospheric fields that respect both the climatological prior and the constraints imposed by meteorological observations.

\subsubsection{Vanilla inpainting and time travel}

The direct replacement does not consider the generated parts of $\mathbf{X}_{t}$, potentially causing incoherence between observed and unobserved regions. To address this, we adopt a rewinding or repaint mechanism that modifies both observed and unobserved regions iteratively, enhancing spatial coherence and adherence to observation constraints \cite{lugmayr2022repaint}.

For any $t \in \Omega$, after replacing observed values, we rewind to an earlier time step $t-\tau$ by sampling $p(\mathbf{X}_{t-\tau} | \mathbf{X}_{t})$. The denoising steps are then repeated from $t-\tau$ to $t$ for $K$ rounds, with observation replacement applied at each round. This iterative process allows joint refinement of both observed and unobserved regions, yielding high-quality samples that balance observation constraints and model priors.

\begin{algorithm}[htbp]
\caption{Inpainting Methodology for GAP}
\label{alg:inpainting}
\begin{algorithmic}[1]
\Require 
\begin{itemize}
    \item Pre-trained diffusion model $p_{\Theta^*}$
    \item Observations $\mathbf{x}_0 \odot \mathbf{m}$
    \item Repainting time step set $\Omega$
    \item Rewinding step $\tau$
    \item Rewinding rounds $K$
\end{itemize}
\Ensure Observation-constrained, spatially coherent sample $\mathbf{x}_0$

\State Initialize $\mathbf{x}_T \sim \mathcal{N}(\mathbf{0}, \mathbf{I})$ \Comment{Random initialization}
\For{$t = T-1, \dots, 1$}
    \State Sample $\mathbf{x}_t \sim p_{\Theta^*}(\mathbf{x}_{t} | \mathbf{x}_{t+1})$ \Comment{Reverse sampling}
    \If{$t \in \Omega$} \Comment{Apply repainting at selected steps}
        \For{$k = 1, \dots, K$} \Comment{Perform $K$ rewinding rounds}
            \State Sample $\mathbf{x}_{t}^{\text{obser}} \sim p(\mathbf{x}_{t} \odot \mathbf{m} | \mathbf{x}_{0} \odot \mathbf{m})$ \Comment{Condition on observed data}
            \State Update $\mathbf{x}_t \gets \mathbf{x}_t \odot (\mathbf{I} - \mathbf{m}) + \mathbf{x}_{t}^{\text{obser}}$
            \State Sample $\mathbf{x}_{t+\tau} \sim p(\mathbf{x}_{t+\tau} | \mathbf{x}_{t})$ \Comment{Rewind by $\tau$ steps}
            \For{$i = t+\tau-1, \dots, t$} \Comment{Denoise over rewinding range}
                \State Sample $\mathbf{x}_i \sim p_{\Theta^*}(\mathbf{x}_{i} | \mathbf{x}_{i+1})$
            \EndFor
        \EndFor
    \EndIf
\EndFor
\State \Return $\mathbf{x}_0$ \Comment{Final reconstructed sample}
\end{algorithmic}
\end{algorithm}

The iterative inpainting methodology ensures that generated samples are spatially coherent and adapt to observation constraints. It is particularly useful in scenarios with sparse observations and varying layouts.

\begin{figure}
\centerline{\includegraphics[width=1\textwidth]{suppli_fig/inpainting_SDE.jpg}}
\caption{A pre-defined forward Gaussian process (left) turns distribution of target climate variable into a prior distribution, i.e., standard Gaussian. A learned reverse Gaussian process (right) turns the prior distribution into the distribution of the target climate variable. We ``inpaint'' sparse observations throughout the reverse Gaussian process (right top), so as to obtain spatial pattern estimates of the target variable. In "SDEdit" part, we add define a forward process based on a forecast to obtain a prior distribution with model forecast.}
\label{fig_inpainting_SDE}
\end{figure}

\subsubsection{Copaint}

Weather scale assimilation and climate reconstruction problem involves generating high-resolution, spatially coherent climate fields from partially observed data. Existing approaches often fail to ensure consistency between observed and unobserved regions, especially in high-dimensional and spatially correlated settings. While traditional inpainting techniques have proven effective for image processing, their direct application to climate data reconstruction suffers from limitations, including lack of physical consistency with climatological constraints, incoherence between observed and reconstructed regions and inability to effectively propagate uncertainty in the reconstructed fields.

In this study, we use a advanced guiding technique called \textbf{Copaint}\cite{zhang2023towards} leveraging diffusion models to address these shortcomings, enabling applications in climate reanalysis and ensemble generation.

Formally, let $r(\cdot)$ be an operator extracting observed values from a climate field, and $s_0$ the observed subset of the reference field. The goal is to generate a complete field $\tilde{X}_0$ satisfying the constraint:

\begin{equation*}
C: r(\tilde{X}_0) = s_0,
\end{equation*}

where $C$ ensures the reconstructed field matches the observations. We utilize pre-trained diffusion models with fixed parameters $f_\theta^{(t)}$ for all $t$. Many existing methods impose constraints by directly replacing observed regions in intermediate or final generated fields, which can lead to inconsistencies. Copaint refines both observed and unobserved regions iteratively for coherence.

Assuming $\sigma_t = 0$ for all $t$, the deterministic DDIM~\cite{song2020denoising} process ensures that $\tilde{X}_0$ is deterministically derived from $\tilde{X}_T$. The posterior distribution becomes:

\begin{equation*}
\begin{split}
p_\theta(\tilde{X}_T | C) &\propto p_\theta(\tilde{X}_T) \cdot \delta(r(\tilde{X}_0) - s_0),
\end{split}
\end{equation*}

where $\delta(\cdot)$ enforces the reconstruction constraint. Taking the logarithm, the posterior distribution simplifies to:

\begin{equation*}
\log p_\theta(\tilde{X}_T | C) \approx -\frac{1}{2} \|\tilde{X}_T\|_2^2 - \frac{1}{2\xi_T^2} \|s_0 - r(g_\theta(\tilde{X}_T))\|_2^2 + C.
\end{equation*}

Gradient-based optimization on $\tilde{X}_T$ yields the maximum a posteriori (MAP) estimate, ensuring consistency across regions.

To reduce computational complexity, we replace $g_\theta(\tilde{X}_T)$ with a one-step approximation $f_\theta^{(T)}(\tilde{X}_T)$:

\begin{equation*}
\log p'_\theta(\tilde{X}_T | C) = -\frac{1}{2} \|\tilde{X}_T\|_2^2 - \frac{1}{2\xi_{T}^2} \|s_0 - r(f_\theta^{(T)}(\tilde{X}_T))\|_2^2 + C',
\end{equation*}

where $\xi'_T$ captures the approximation error, balancing accuracy and computational feasibility.

To iteratively refine the reconstruction, we adopt a non-deterministic DDIM procedure with $\sigma_t \neq 0$. The approximate posterior is:

\begin{equation*}
p'_\theta(\tilde{X}_{0:T}|C) = p'_\theta(\tilde{X}_T|C) \prod_{t=1}^{T} p'_\theta(\tilde{X}_{t-1}|\tilde{X}_t, C),
\end{equation*}

where intermediate steps are corrected by optimizing:

\begin{equation*}
\log p'_\theta(\tilde{X}_{t-1}|\tilde{X}_t, C) = -\frac{1}{2\sigma_t^2} \|\tilde{X}_{t-1} - \mu_t\|_2^2 - \frac{1}{2\xi_t'^2} \|s_0 - r(f_\theta^{(t)}(\tilde{X}_{t-1}))\|_2^2 + C'.
\end{equation*}

This methodology demonstrates significant potential in weather and climate modeling, enabling high-resolution field generation consistent with sparse observational data. Future applications include data assimilation, reanalysis, and emulation of climate ensembles.

\subsection{SDEdit}\label{SDEdit}

\subsubsection{Formulation}

Stochastic Differential Equation Editing (SDEdit) is a guided synthesis framework that leverages generative stochastic differential equations to improve forecast quality\cite{meng2021sdedit}. In GAP's formula, it begins with three key components:
\begin{enumerate}
    \item A learned climatological prior in the form of a probabilistic diffusion model, which approximates $p_{\theta^*}(\mathbf{X}|\Theta)$
    \item A sample of atmospheric state estimate at time $t$, $\mathbf{X}_t$
    \item A forecasting model $\mathcal{M}$ that maps $\mathbf{X}_t$ to predicted state $\mathbf{X}_{t+\Delta t}$
\end{enumerate}

The forecasting model inevitably contains both systematic biases $\mathbf{b}$ and stochastic uncertainties $\boldsymbol{\epsilon}$, such that:
\begin{equation*}
    \mathcal{M}(\mathbf{X}_t) = \mathbf{X}_{t+\Delta t} + \mathbf{b} + \boldsymbol{\epsilon}
\end{equation*}
where $\mathbb{E}[\boldsymbol{\epsilon}] = \mathbf{0}$ and $\text{Cov}(\boldsymbol{\epsilon}) = \boldsymbol{\Sigma}_{\text{random}}$.

Our objective is to obtain the probabilistic distribution of the next time step atmospheric state $\mathbf{X}_{t+\Delta t}$ by combining the predictive information from $\mathcal{M}(\mathbf{X}_t)$ with the climatological constraints from the diffusion model.

The SDEdit framework leverages the learned climatological prior through a two-step process:
\begin{enumerate}
    \item \textbf{Forward diffusion}: Add calibrated noise to the model's prediction $\mathcal{M}(\mathbf{X}_t)$ by running the forward SDE from $\tau = 0$ to $\tau^*$ with initial condition $\mathbf{x}_{\tau=0} = \mathcal{M}(\mathbf{X}_t)$
    \item \textbf{Reverse diffusion}: Run the reverse SDE back to $\tau = 0$ to generate the probabilistic estimate for $\mathbf{X}_{t+\Delta t}$
\end{enumerate}

We denote the result of this process as $\text{SDEdit}(\mathcal{M}(\mathbf{X}_t), \tau^*)$.

\subsubsection{Error Analysis}

To determine the optimal noise level $\tau^*$, we analyze the expected error between the true state $\mathbf{X}_{t+\Delta t}$ and the SDEdit estimate. The squared $L_2$ error can be bounded as:
\begin{equation*}
\begin{aligned}
\|\mathbf{X}_{t+\Delta t} - \text{SDEdit}(\mathcal{M}(\mathbf{X}_t), \tau^*)\|_2^2 &\leq \|\mathbf{X}_{t+\Delta t} - \text{SDEdit}(\mathbf{X}_{t+\Delta t}, \tau^*)\|_2^2 \\
&+ \|\text{SDEdit}(\mathbf{X}_{t+\Delta t}, \tau^*) - \text{SDEdit}(\mathcal{M}(\mathbf{X}_t), \tau^*)\|_2^2
\end{aligned}
\end{equation*}

This inequality decomposes the prediction error into two components:
\begin{enumerate}
    \item \textbf{Diffusion Process Error}: The inherent information loss from applying noise at level $\tau^*$ to the true state
    \item \textbf{Error Propagation}: How differences between the true future state and model prediction propagate through the diffusion process
\end{enumerate}

\subsubsection{Diffusion Process Error}

For the diffusion process error term, we consider a variance-preserving diffusion model with a linear noise schedule. The forward process is defined by the stochastic differential equation:
\begin{equation*}
d\mathbf{x} = -\frac{1}{2}\beta(t)\mathbf{x}dt + \sqrt{\beta(t)}d\mathbf{w}
\end{equation*}
where:
\begin{itemize}
    \item $\mathbf{x}$ is the state variable evolving through diffusion time
    \item $\beta(t)$ is the noise schedule function that determines diffusion rate
    \item $\mathbf{w}$ is the standard Wiener process (Brownian motion)
    \item $t$ is the diffusion time parameter (denoted as $\tau$ in our context)
\end{itemize}

For a linear noise schedule, $\beta(t) = \beta_{\min} + t(\beta_{\max} - \beta_{\min})/T$ where $T$ is the maximum diffusion time, and typically $\beta_{\min} \ll \beta_{\max}$.

Starting from the initial condition $\mathbf{x}_0 = \mathbf{X}_{t+\Delta t}$ (our true atmospheric state), the state at diffusion time $\tau$ follows:
\begin{equation*}
\mathbf{x}_\tau = \alpha(\tau)\mathbf{x}_0 + \sqrt{1-\alpha(\tau)^2}\boldsymbol{\epsilon}
\end{equation*}
where:
\begin{itemize}
    \item $\alpha(\tau) = e^{-\frac{1}{2}\int_0^\tau \beta(s)ds} \approx e^{-\tau}$ (for appropriate scaling of $\beta$)
    \item $\boldsymbol{\epsilon} \sim \mathcal{N}(\mathbf{0}, \mathbf{I})$ is a standard normal noise vector
\end{itemize}

For a perfect diffusion model that exactly learns the score function of the data distribution, the expected output of SDEdit is:
\begin{equation*}
\mathbb{E}[\text{SDEdit}(\mathbf{X}_{t+\Delta t}, \tau^*)] = \mathbf{X}_{t+\Delta t}
\end{equation*}

However, the actual output will have variance due to stochasticity in both forward and reverse processes:
\begin{equation*}
\text{Var}[\text{SDEdit}(\mathbf{X}_{t+\Delta t}, \tau^*)] = (1 - e^{-2\tau^*})\boldsymbol{\Sigma}_{\text{prior}}
\end{equation*}
where $\boldsymbol{\Sigma}_{\text{prior}}$ is the covariance matrix of the climatological distribution learned by the diffusion model.

The factor $(1 - e^{-2\tau^*})$ quantifies the degree of information loss, which increases monotonically with $\tau^*$. Given this variance, the expected squared error is:
\begin{equation*}
\mathbb{E}[\|\mathbf{X}_{t+\Delta t} - \text{SDEdit}(\mathbf{X}_{t+\Delta t}, \tau^*)\|_2^2] = \text{tr}((1 - e^{-2\tau^*})\boldsymbol{\Sigma}_{\text{prior}})
\end{equation*}

This error increases from zero (when $\tau^* = 0$) to $\text{tr}(\boldsymbol{\Sigma}_{\text{prior}})$ (when $\tau^* \rightarrow \infty$).

\subsubsection{Error Propagation}

Assuming Lipschitz continuity of the SDEdit operator with constant $L(\tau^*) = e^{-\tau^*}$:
\begin{equation*}
\|\text{SDEdit}(\mathbf{X}_{t+\Delta t}, \tau^*) - \text{SDEdit}(\mathcal{M}(\mathbf{X}_t), \tau^*)\|_2^2 \leq e^{-2\tau^*} \|\mathbf{X}_{t+\Delta t} - \mathcal{M}(\mathbf{X}_t)\|_2^2
\end{equation*}

This term decreases exponentially with $\tau^*$, representing how the diffusion process progressively "forgets" the input as more noise is added.

The total error bound is therefore:
\begin{equation*}
\|\mathbf{X}_{t+\Delta t} - \text{SDEdit}(\mathcal{M}(\mathbf{X}_t), \tau^*)\|_2^2 \leq \text{tr}((1 - e^{-2\tau^*})\boldsymbol{\Sigma}_{\text{prior}}) + e^{-2\tau^*} \|\mathbf{X}_{t+\Delta t} - \mathcal{M}(\mathbf{X}_t)\|_2^2
\end{equation*}

\subsubsection{Model Error Decomposition}

To better understand when SDEdit outperforms raw model predictions, we decompose the model error, separating systematic bias from random errors:
\begin{equation*}
\mathcal{M}(\mathbf{X}_t) = \mathbf{X}_{t+\Delta t} + \mathbf{b} + \boldsymbol{\epsilon}
\end{equation*}

The raw model squared error is:
\begin{equation*}
\|\mathbf{X}_{t+\Delta t} - \mathcal{M}(\mathbf{X}_t)\|_2^2 = \|\mathbf{b}\|_2^2 + \|\boldsymbol{\epsilon}\|_2^2
\end{equation*}

A key property of the diffusion model is its ability to correct systematic biases. We can model the SDEdit output as:
\begin{equation*}
\text{SDEdit}(\mathcal{M}(\mathbf{X}_t), \tau^*) \approx \mathbf{X}_{t+\Delta t} + c(\tau^*)\mathbf{b} + d(\tau^*)\boldsymbol{\epsilon} + \boldsymbol{\eta}(\tau^*)
\end{equation*}

where:
\begin{itemize}
    \item $c(\tau^*)$ modulates the remaining bias (with $0 \leq c(\tau^*) \leq 1$)
    \item $d(\tau^*)$ modulates the random error component (with $0 \leq d(\tau^*) \leq 1$)
    \item $\boldsymbol{\eta}(\tau^*)$ is the noise introduced by the diffusion process with $\text{Cov}(\boldsymbol{\eta}(\tau^*)) = \boldsymbol{\Sigma}_{\text{diff}}(\tau^*)$
\end{itemize}

Importantly, $c(\tau^*)$ typically decreases faster than $d(\tau^*)$ because systematic biases are easier to correct than random errors. Both $c(\tau^*)$ and $d(\tau^*)$ are decreasing functions of $\tau^*$, while $\boldsymbol{\Sigma}_{\text{diff}}(\tau^*)$ is an increasing function of $\tau^*$.

The expected squared error for SDEdit becomes:
\begin{equation*}
\mathbb{E}[\|\mathbf{X}_{t+\Delta t}-\text{SDEdit}(\mathcal{M}(\mathbf{X}_t), \tau^*)\|_2^2] = \|c(\tau^*)\mathbf{b}\|_2^2+\|d(\tau^*)\|_2^2\text{tr}(\boldsymbol{\Sigma}_{\text{random}})+ \text{tr}(\boldsymbol{\Sigma}_{\text{diff}}(\tau^*))
\end{equation*}

\subsubsection{Comparison with Raw Model Error}

SDEdit outperforms raw model prediction when:
\begin{equation*}
\|c(\tau^*)\mathbf{b}\|_2^2 + \|d(\tau^*)\|_2^2\text{tr}(\boldsymbol{\Sigma}_{\text{random}}) + \text{tr}(\boldsymbol{\Sigma}_{\text{diff}}(\tau^*)) < \|\mathbf{b}\|_2^2 + \text{tr}(\boldsymbol{\Sigma}_{\text{random}})
\end{equation*}

This can be rewritten as:
\begin{equation*}
\text{tr}(\boldsymbol{\Sigma}_{\text{diff}}(\tau^*)) < (1 - \|c(\tau^*)\|_2^2)\|\mathbf{b}\|_2^2 + (1 - \|d(\tau^*)\|_2^2)\text{tr}(\boldsymbol{\Sigma}_{\text{random}})
\end{equation*}

This inequality reveals that SDEdit can outperform raw model predictions even when the climatological variance exceeds model error, particularly when:
\begin{enumerate}
    \item The model has significant systematic biases ($\|\mathbf{b}\|_2^2$ is large)
    \item The noise level $\tau^*$ is chosen to maximize bias correction while minimizing diffusion noise
    \item The diffusion process efficiently corrects biases relative to how quickly it introduces its own uncertainty
\end{enumerate}

\subsubsection{Optimal Noise Level}

The optimal noise level $\tau^*$ minimizes the expected error:
\begin{equation*}
\tau^* = \arg\min_{\tau} \left[\|c(\tau)\mathbf{b}\|_2^2 + \|d(\tau)\|_2^2\text{tr}(\boldsymbol{\Sigma}_{\text{random}}) + \text{tr}(\boldsymbol{\Sigma}_{\text{diff}}(\tau))\right]
\end{equation*}

This optimization problem typically yields a U-shaped error curve with respect to $\tau$, suggesting an optimal noise level that balances:
\begin{itemize}
    \item Bias correction (improved with increasing $\tau$)
    \item Random error retention (reduced with increasing $\tau$)
    \item Diffusion noise introduction (increased with increasing $\tau$)
\end{itemize}

Under simplified assumptions where $c(\tau) \approx e^{-\alpha\tau}$, $d(\tau) \approx e^{-\beta\tau}$ with $\alpha > \beta$, and $\boldsymbol{\Sigma}_{\text{diff}}(\tau) \approx (1 - e^{-2\tau})\boldsymbol{\Sigma}_{\text{prior}}$, the optimal $\tau^*$ can be approximated as:
\begin{equation*}
\tau^* \approx \frac{1}{2\alpha} \ln \left( \frac{2\alpha\|\mathbf{b}\|_2^2}{\text{tr}(\boldsymbol{\Sigma}_{\text{prior}})} \right)
\end{equation*}

This formula demonstrates that the optimal noise level:
\begin{itemize}
    \item Increases with larger systematic bias $\|\mathbf{b}\|_2^2$
    \item Decreases with larger climatological variance $\text{tr}(\boldsymbol{\Sigma}_{\text{prior}})$
    \item Scales inversely with the bias correction efficiency $\alpha$
\end{itemize}

\subsubsection{Implementation Details}

In practice, the forward and reverse diffusion processes are defined as follows:
\begin{align*}
q(x_t|x_{t-1}) &= \mathcal{N}(x_t; \sqrt{1 - \beta_t} x_{t-1}, \beta_t \mathbf{I}), \\
p_{\Theta}(x_{t-1}|x_t) &= \mathcal{N}(x_{t-1}; \mu_{\Theta}(x_t), \Sigma_{\Theta}(x_t)),
\end{align*}
where $\beta_t$ denotes the noise schedule, and $\mu_{\Theta}$, $\Sigma_{\Theta}$ are the mean and variance learned by the model.

The reverse SDE is defined as:
\begin{align*}
\mathrm{d}\mathbf{X} &= \left[\mathbf{f}(\mathbf{X}, t) - g(t)^2 \nabla_{\mathbf{X}} \log p_t(\mathbf{X})\right] \mathrm{d}t + g(t)\mathrm{d}\bar{\mathbf{w}},
\end{align*}
where $\mathbf{f}(\mathbf{X}, t)$ is the drift term, $g(t)$ is the noise coefficient, and $p_t(\mathbf{X})$ represents the probability density.

The model parameters $\boldsymbol{\Theta}$ are optimized by minimizing the expected difference between model and data gradients:
\begin{align*}
    \boldsymbol{\Theta}^{*} = \underset{\boldsymbol{\Theta}}{\operatorname*{arg\,min}} \mathbb{E}_t \Big\{ \lambda(t) \mathbb{E}_{\mathbf{X}(0)} \mathbb{E}_{\mathbf{X}(t)|\mathbf{X}(0)} \Big[ \| \mathbf{s}_{\boldsymbol{\Theta}}(\mathbf{X}(t), t) - \nabla_{\mathbf{X}(t)} \log p_{0t}(\mathbf{X}(t)|\mathbf{X}(0)) \|_2^2 \Big] \Big\}.
\end{align*}

\subsubsection{Theoretical Bounds on Noise Level}

For practical implementation, determining the appropriate noise level $t_0$ is critical. We establish theoretical bounds on $t_0$ as follows:

For the upper bound, $t_0$ must be small enough that $x_{t_0}$ from either the model or reality, after diffusion, become identically distributed. For the lower bound, $t_0$ must be large enough that the denoising result error is comparable to the original model error:

\begin{align*}
    ||\mathbf{X}_{t_{i}}-\text{SDEdit}(\mathbf{M}(\mathbf{X}_{t_{i-1}}),\tau)||^2_2 \leq 
    ||\mathbf{X}_{t_{i}}-\text{SDEdit}(\mathbf{X}_{t_{i}},\tau)||^2_2 + \\
    ||\text{SDEdit}(\mathbf{X}_{t_{i}},\tau)-\text{SDEdit}(\mathbf{M}(\mathbf{X}_{t_{i-1}}),\tau)||^2_2.
\end{align*}

For the lower bound term $||\mathbf{X}_{t_{i}}-\text{SDEdit}(\mathbf{X}_{t_{i}},\tau)||^2_2$, assuming $\|s_\theta(\mathbf{x}, t)\|_2^2 \leq C$ for all $\mathbf{x} \in \mathcal{X}$ and $t \in [0,1]$, then for all $\delta \in (0,1)$ with probability at least $(1-\delta)$:

\begin{align*}
    \|\mathbf{x}^{(g)} - \text{SDEdit}(\mathbf{x}^{(g)}; t_0, \theta)\|_2^2 \leq \sigma^2(t_0)(C\sigma^2(t_0) + d + 2\sqrt{-d \cdot \log \delta} - 2\log \delta)
\end{align*}

where $d$ is the dimensionality of $\mathbf{x}^{(g)}$.

For the upper bound to ensure identically distributed variables after adding noise, we consider two random variables:
\[ y_1 = X_1 + g(t)Z \]
\[ y_2 = X_2 + g(t)Z \]
where $X_2 = X_1 + \epsilon$, $\epsilon \sim f$, and $Z$ is standard normal.

For $y_1$ and $y_2$ to be identically distributed, we must have:
\[ g(t) \geq \frac{\sigma_f}{\sqrt{2}} \]
where $\sigma_f^2$ is the variance of distribution $f$.

This bound is tight, representing the minimum amount of Gaussian noise needed to dominate the variance of the original difference distribution $f$. This result implies that the required magnitude of $g(t)$ increases with the standard deviation of $f$.

In our empirical validation (SI Section \ref{choice_of_noise_level}), we conducted experiments measuring the error as a function of $\tau^*$ for various atmospheric variables and forecast lead times. The results confirmed the predicted U-shaped error curves and aligned well with our theoretical optimal $\tau^*$ values.

\subsection{Seasonal prediction settings}\label{Seasonal_prediction_settings}

\subsubsection{Overview}

The chaotic nature of atmospheric processes fundamentally limits weather predictability \cite{lorenz1963deterministic}. Small uncertainties in initial conditions amplify exponentially over time due to the nonlinear dynamics of the atmosphere, resulting in a theoretical predictability limit of approximately two weeks \cite{zhang2019predictability}. This inherent limitation, coupled with the atmosphere's rapid response to various forcings and its high-dimensional degrees of freedom, makes purely atmospheric prediction beyond this timescale particularly challenging \cite{buizza2015forecast}. To address this challenge, slowly evolving climate components, such as the ocean and land systems, are leveraged to constrain uncertainty growth and extend predictability.

As a compelling example, we highlight how GAP integrates sea surface temperature (SST) to incorporate key Earth system components, demonstrating its potential to enhance predictability beyond the limits of purely atmospheric forecasts. SST has strong correlation with atmospheric component like 2m temperature, particcularly evident in tropical regions and areas of strong air-sea interaction \cite{czaja2011new}. As a thermal forcing for atmospheric circulation, SST is a especially robust indicator on seasonal timescales \cite{krishnamurthy2019predictability, deser2010sea}, where SST anomalies can explain up to 30-40\% of 2m temperature variance in key regions such as the North Atlantic and tropical Pacific \cite{peng2005tropical}.

Leveraging the ocean's longer persistence timescale \cite{von2002statistical}, we incorporate SST anomaly persistence as an additional constraint within GAP's seamless prediction framework. Specifically, we establishing a mapping relationship between SST and 2m temperature fields. The 2m temperature fields predicted based on SST persistence are then seamlessly integrated into GAP using inpainting techniques.

\subsubsection{Sea surface temperature anomaly persistence}\label{SAP}

The Sea Surface Temperature (SST) Anomaly Persistence (SAP) prediction method for SST represents a simplified oceanic forecasting framework that operates on the fundamental assumption of temporal stability in SST anomaly patterns relative to their climatological baseline (SI Fig. \ref{fig_SAP_schematic}). This approach leverages the inherent temporal persistence of SST fields, utilizing known SST anomalies and climatological values at time $t = 0$ to project future thermal states.  Given the characteristic slow evolution of SST fields, the APP method demonstrates particular efficacy in preserving the spatial coherence of temperature distributions over short-term forecast horizons. Therefore, the SAP method plays an important role in the prediction of ocean elements in the early stage of the development of the sea-air coupling model. However, the methodology exhibits notable limitations: primarily, its inability to adequately capture underlying physical mechanisms and the challenge of representing inter-spatial dynamics in the prediction framework.  These constraints significantly impact the model's capacity to generate physically consistent forecasts that account for spatial teleconnections and complex ocean-atmosphere interactions.

\begin{figure}
\centering
\includegraphics[width=0.6\linewidth]{suppli_fig/SAP_schematic.pdf}
\caption{A schematic of SST Anomaly Persistence Prediction method.}
\label{fig_SAP_schematic}
\end{figure}

\subsubsection{Mapping from SST to 2m temperature}\label{map_sst_t2m}

Extensive research highlights the strong relationship between sea surface temperature (SST) and 2-meter temperature (t2m), with several simple statistical models mapping SST to t2m \cite{czaja2011new, peng2005tropical, yu2006variance}. In this study, we directly train a simple neural network to efficiently perform this mapping within the GAP workflow.

We employ a vanilla U-Net model to establish the mapping between SST and t2m fields, adopting a Maximum Likelihood Estimation approach. The encoder path begins with a $3\times3$ convolution that expands the single SST channel into 128 feature channels, followed by a series of residual blocks (ResBlocks) that maintain the channel width. Each ResBlock consists of a sequence of convolution, batch normalization, ReLU activation, another convolution, and batch normalization, supplemented by a skip connection to preserve the input. Dropout ($p=0.1$) is applied for regularization. The decoder path mirrors the encoder, incorporating skip connections from corresponding encoder levels to retain spatial details. The network outputs the mean and variance of the t2m fields through two parallel $1\times1$ convolution layers.

The model is trained using a sliding window approach over 5-year cycles (1990–2019), where 4 years are allocated for training and 1 year for validation. This temporal splitting strategy mitigates the influence of long-term global warming trends, ensuring the model focuses on day-to-day variations rather than gradual climate shifts. Training employs the Adam optimizer with an initial learning rate of $1 \times 10^{-5}$ and a batch size of 128. Early stopping is implemented with a patience of 50 epochs and a delta of $1 \times 10^{-4}$, along with a linear learning rate decay schedule. To further prevent overfitting, training is capped at a maximum of 200 epochs.

\subsection{Climate simulation settings}\label{Climate_simulation_settings}

For climate simulation and projection, we implemented GAP in two primary configurations: a free-running setup without external constraints and a boundary-forced setup incorporating prescribed external forcings. In the free-running configuration, GAP evolves autonomously from initial conditions sampled from the climatological prior, with no additional constraints on sea surface temperatures (SST) or other boundary fields. This setup allows GAP to generate internally consistent atmospheric states driven solely by its learned probabilistic dynamics. The model samples weather trajectories directly from the learned prior, capturing the intrinsic variability of the climate system over long timescales.

In the boundary-forced configuration, external climate forcings—such as SSTs representing ocean heat content—are introduced as conditions using inpainting during the generative process. Specifically, at each time step, SST fields from an external source (e.g., reanalysis data or climate model projections) are prescribed, and the inpainting technique is applied within the diffusion process to condition the atmospheric state on these boundary values. This approach allows GAP to flexibly integrate boundary constraints without requiring retraining, effectively embedding oceanic influences into the probabilistic sampling process. For climate projections, we prescribed SST fields from CESM2 future scenario simulations under different Shared Socioeconomic Pathways (SSP1-2.6, SSP3-7.0, SSP5-8.5) as boundary conditions.

The incorporation of external forcings follows the Bayesian framework described in Eq. \ref{bayes}, where the likelihood term $p(\mathbf{O}_i|\mathbf{X}_i, \Theta)$ is adapted to represent the deviation of the atmospheric state from the prescribed SSTs. This is achieved by treating SST as an observation and applying inpainting to ensure the sampled atmospheric fields remain consistent with the boundary condition. This flexible conditioning mechanism enables GAP to perform conditional probabilistic inference while maintaining physical coherence across atmospheric and oceanic variables, facilitating both transient projections and long-term equilibrium climate simulations.

\subsection{Choice of noise level}\label{choice_of_noise_level}

An important hyperparameter in the GAP model is the selection of the noise level, \( t_0 \), especially when using biased forecasts or analyses as conditional inputs. This parameter plays a critical role in balancing the fidelity to the conditional input and the stochastic variability. In section \ref{SDEdit}, we give the theoretical denotation. Practically, Hess et al. \cite{hess2024fast} introduced a novel criterion for determining \( t_0 \) in meteorology-based applications using power spectrum analysis, providing a robust methodology to ensure consistency in model behavior across scales.

As an illustrative example, we calculate the specific humidity at 850 hPa for various noise levels (Fig.~\ref{fig_Noise_level_PSD_comparison_ERA5_forecast}). The total number of noise steps is set to 160. When the noise level \( t_0 \) approaches the total steps (indicating strong fidelity to the conditional input), the power spectrum exhibits inconsistencies at small scales. These discrepancies have also been highlighted in recent evaluations of machine-learning-based models \cite{bonavita2024some}, emphasizing their significance. 

By increasing the number of noise steps, these small-scale inconsistencies are progressively reduced. At approximately 80 noise steps, the power spectrum aligns closely with the reference, demonstrating that this level achieves a suitable balance between stochasticity and conditional faithfulness. This behavior indicates that \( t_0 = 80 \) is a reasonable choice for this setup.

% \begin{figure}
% \centerline{\includegraphics[width=1\textwidth]{suppli_fig/inpainting_SDE.jpg}}
% \caption{A pre-defined forward Gaussian process (left) turns distribution of target climate variable into a prior distribution, i.e., standard Gaussian. A learned reverse Gaussian process (right) turns the prior distribution into the distribution of the target climate variable. We ``inpaint'' sparse observations throughout the reverse Gaussian process (right top), so as to obtain spatial pattern estimates of the target variable. In "SDEdit" part, we add define a forward process based on a forecast to obtain a prior distribution with model forecast.}
% \label{fig_inpainting_SDE}
% \end{figure}

\begin{figure}
\centering
\includegraphics[width=1\linewidth]{suppli_fig/PSD_nise_level_supplifig_V1.pdf}
\caption{Power spectral density (PSD) maps for specific humidity at 850 hPa under different noise levels, using ERA5 and forecast fields.}
\label{fig_Noise_level_PSD_comparison_ERA5_forecast}
\end{figure}

To ensure that all 69 atmospheric variables in the GAP model are calibrated appropriately, we introduce an additional evaluation criterion according to section \ref{SDEdit}. Each variable exhibits unique power spectral characteristics, necessitating a comprehensive approach. We calculate the normalized mean absolute error (MAE) for all variables under different noise levels. As shown in Fig.~\ref{fig_Noise_level_mae_comparison_ERA5_forecast}, the MAE decreases as noise steps increase. When the noise level is around 80 steps, the MAE reduces to an acceptable range (less than \( 1 \times 10^{-3} \) for the mean value), confirming the suitability of \( t_0 = 80 \). However, for noise levels larger than 80, the MAE increases again, indicating a trade-off between noise injection and conditional fidelity.

Based on these results, we recommend setting \( t_0 = 80 \) when the total noise steps are 160 in most cases. Nevertheless, specific scenarios may require fine-tuning of the noise level to accommodate particular conditions or to achieve the desired balance between stochasticity and model fidelity. This highlights the importance of tailoring \( t_0 \) for optimal model performance across a wide range of applications.

\begin{figure}[H]
\centering
\includegraphics[width=0.8\linewidth]{suppli_fig/Noise_level_mae_comparison_ERA5_forecast_suppli.pdf}
\caption{Normalized mean absolute error (MAE) comparison for all 69 atmospheric variables under different noise levels, using ERA5 and forecast data.}
\label{fig_Noise_level_mae_comparison_ERA5_forecast}
\end{figure}

\clearpage

\section{Statistical methods}\label{Appendix_evaluation_metrics}

\subsection{Determinstic metrics}\label{Determinstic_metrics}

\subsubsection{Root mean square error (RMSE)}

When the predicted meteorological field of $A_t$ is available at time $t = t_0 + \Delta t$, denoted as $\hat{A}_t$, we compute the Root Mean Square Error (RMSE) as follows:

\begin{equation*}
\text{RMSE}(\nu, t) = \sqrt{
    \frac{
        \sum_{i=1}^{N_{\text{lat}}} \sum_{j=1}^{N_{\text{lon}}} L(i) \left( \hat{A}_{i,j,t}^\nu - A_{i,j,t}^\nu \right)^2
    }{
        N_{\text{lat}} \times N_{\text{lon}}
    }
},
\end{equation*}

where $N_{\text{lat}}$ and $N_{\text{lon}}$ represent the number of latitude and longitude grid points, respectively. The weight at latitude $L(i)$ is given by
\begin{equation*}
L(i) = N_{\text{lat}} \times \frac{\cos \phi_i}{\sum_{i=1}^{N_{\text{lat}}} \cos \phi_i},
\end{equation*}
where $N_{\text{lat}}$ and $N_{\text{lon}}$ denote the number of latitude and longitude grid points, respectively.

\subsubsection{Anomaly correlation coefficient (ACC)}

The Anomaly Correlation Coefficient (ACC) is one of the most widely used measures for verifying spatial fields. It quantifies the spatial correlation between forecast anomalies relative to climatology and verifying analysis anomalies relative to climatology. ACC measures how well forecast anomalies represent observed anomalies, indicating how accurately the predicted values from a forecast model align with ground truth data. For a series of forecast lead times, ACC evaluates how well trends in predicted anomalies follow trends in actual anomalies.

\begin{equation*}
\text{ACC}(\nu, t) = \frac{
    \sum_{i=1}^{N_{\text{lat}}} \sum_{j=1}^{N_{\text{lon}}} L(i) \hat{A}_{i,j,t}^\nu A_{i,j,t}^\nu
}{
    \sqrt{
        \sum_{i=1}^{N_{\text{lat}}} \sum_{j=1}^{N_{\text{lon}}} L(i) \left( \hat{A}_{i,j,t}^\nu \right)^2 \times 
        \sum_{i=1}^{N_{\text{lat}}} \sum_{j=1}^{N_{\text{lon}}} L(i) \left( A_{i,j,t}^\nu \right)^2
    }
}
\end{equation*}

Here, $\nu$ represents any weather variable, and $A_{i,j,t}^\nu$ is the value of $\nu$ at time $t$ and horizontal coordinate $(i,j)$. The anomaly $\hat{A}'$ denotes the difference between $A$ and climatology, which is the long-term mean of weather states estimated from 39 years of training data.
%Additionally, these metrics can be evaluated for specific regions, such as the Northern Hemisphere, the Southern Hemisphere, and the tropics.

\subsubsection{Relative skill}\label{clim_relative_rmse_dis}

The evaluation of the model's relative skill is based on normalized Root Mean Squared Error (RMSE), enabling comparisons across different variables and atmospheric layers. To assess the relative error of the climatology, the RMSE is computed after normalizing all variables, ensuring a fair comparison across different variables.

For the assimilation skill assessment, the relative skill of GAP is determined by comparing its RMSE with that of IFS-HRES, both evaluated against the ground truth. Specifically, the relative skill is quantified as the relative RMSE difference between GAP and IFS-HRES:
\begin{equation*}
\text{Relative Improvement} = \frac{\text{RMSE}_a - \text{RMSE}_b}{\text{RMSE}_b} \times 100\%
\end{equation*}
This metric reflects the percentage by which GAP improves upon (negative values) or lags behind (positive values) the baseline model in reproducing ground truth.

\subsection{Probabilistic metrics}\label{Probabilistic_metrics}

\subsubsection{Continuous ranked probability score (CRPS)}

The Continuous Ranked Probability Score (CRPS; \cite{gneiting2007strictly}) is a standard measure for evaluating the skill of probabilistic forecasts. It assesses how well the marginal distributions of the forecast align with the ground truth, minimizing the score when the forecast distribution matches the truth.

Unlike RMSE, which is minimized when $X(t) = \mathbb{E}[Y(t)]$, CRPS is minimized when the forecast distribution $X(t)$ matches the true distribution $Y(t)$. To define CRPS, consider a ground truth scalar random variable $V$ and two independent forecasts $U$ and $U'$:

\begin{equation*}
\text{CRPS} = \mathbb{E}|U - V| - \frac{1}{2} \mathbb{E}|U - U'|.
\end{equation*}

The skill term $\mathbb{E}|U - V|$ penalizes deviations from the ground truth, while the spread term $\frac{1}{2} \mathbb{E}|U - U'|$ encourages well-dispersed forecasts. CRPS is minimized when $U$ and $V$ share the same distribution \cite{gneiting2007strictly}.

To extend CRPS to multiple dimensions, we sum over components and estimate the score using $M$ ensemble members $(X^{(1)}, \ldots, X^{(M)})$:

\begin{equation*}
\begin{split}
\mathcal{E}_{CRPS}& _{s}(\tau,v,p):= \\
&\frac1{|\mathcal{T}|}\sum_{t\in\mathcal{T}}\frac1{IJ}\sum_{i=1}^{121}\sum_{j=1}^{240}w(i)\left[\right. \\
&\frac{1}{M}\sum_{m=1}^{M}\big|X^{(m)}(t\to t+\tau,v,p,i,j)-Y(t+\tau,v,p,i,j)\big| \\
&\left.-\frac1{2M(M-1)}\sum_{m,k=1}^M\left|X^{(m)}(t\to t+\tau,v,p,i,j)-X^{(k)}(t\to t+\tau,v,p,i,j)\right|\right]
\end{split}
\end{equation*}

The resultant CRPS is minimized when the forecast distribution $X$ matches the true distribution $Y$. This property ensures that CRPS does not penalize correct forecasts but instead evaluates the probabilistic skill of the forecasting system.

% For ensemble weather forecasts, CRPS is computed using tools like the xskillscore Python package. It can also be combined with weather-climate generation models like GAP to assess the fidelity of forecasts across different regions and scales. Mathematically, CRPS is defined as:

% \begin{equation}
% \text{CRPS} = \int_{-\infty}^{+\infty} \left[ F(\hat{A}^{u}_{i,j,t}) - \mathbb{I}(\hat{A}^{u}_{i,j,t} \leq z) \right] dz,
% \end{equation}

% where $F(\cdot)$ is the cumulative distribution function of the forecast distribution, and $\mathbb{I}(\cdot)$ is the indicator function. The integration ensures that the score captures the full probabilistic range of the forecast distribution.

\subsubsection{Continuous Ranked Probability Skill Score (CRPSS)}

The Continuous Ranked Probability Skill Score (CRPSS) is a skill score version of the Continuous Ranked Probability Score (CRPS), which provides a comparison of the forecast performance against a climatology benchmark. It is defined as:

\[
\text{CRPSS} = 1 - \frac{\text{CRPS}_{\text{fc}}}{\text{CRPS}_{\text{bench}}}
\]

where $\text{CRPS}_{\text{fc}}$ is the CRPS of the forecast. $\text{CRPS}_{\text{bench}}$ is the CRPS of the climatology benchmark.

A CRPSS value of 1 indicates a perfect forecast, while values of $\text{CRPSS} > 0$ indicate forecasts that are more skillful than the climatology benchmark. The CRPS of the climatology is computed using a 39-year climatological sample (1979-2018) derived from reanalysis data.

\subsubsection{Spread-skill ratio (SSR)}

The spread-skill ratio (SSR) is a key diagnostic metric that evaluates the reliability of ensemble forecasts by comparing the ensemble spread (a measure of forecast uncertainty) to the forecast skill (root-mean-square error, RMSE). For a generic scalar ground truth $Y_t$ and an ensemble of forecasts $\{X_t^{(n)}\}_{n=1}^{N}$, provided at times $t = 1, \ldots, T$, the ensemble mean and spread are defined as follows:
\[
\mu_t := \frac{1}{N} \sum_{n=1}^{N} X_t^{(n)}, \quad 
S^2 := \frac{1}{T} \sum_{t=1}^{T} \frac{1}{N-1} \sum_{n=1}^{N} (X_t^{(n)} - \mu_t)^2.
\]

The RMSE of the ensemble mean relative to the ground truth is given by:
\[
\epsilon^2 := \frac{1}{T} \sum_{t=1}^{T} \frac{1}{N} \sum_{n=1}^{N} (Y_t - \mu_t)^2.
\]

While $S^2$ provides an unbiased estimate of ensemble variance, the RMSE $\epsilon^2$ is inherently biased, overestimated by a term proportional to the ensemble variance divided by $N$. To correct this, we adjust the RMSE by subtracting $S^2/N$. The adjusted spread-skill ratio is then expressed as:
\[
\text{SSR} = \sqrt{\frac{S^2}{\epsilon^2 - S^2/N}}.
\]

For a perfectly reliable ensemble, where ensemble members $X_t^{(n)}$ are distributed identically to the ground truth $Y_t$, the SSR should equal 1.0. GAP’s ensemble forecasting framework leverages its generative capabilities to enhance the reliability and accuracy of ensemble forecasts, which directly improves the SSR.

\subsection{Energy spectra}\label{energy_spectral}

The zonal spectral energy along lines of constant latitude is computed as a function of wavenumber (unitless), frequency (m$^{-1}$), and wavelength (m). For discrete values $f_l$ along a zonal circle of constant latitude with circumference $C$, the Discrete Fourier Transform (DFT) $F_k$ is defined as:
\begin{equation*}
    F_k = \frac{1}{L} \sum_{l=0}^{L-1} f_l e^{-i2\pi kl / L},
\end{equation*}
where $L$ is the total number of samples.

The energy spectrum is then given by:
\begin{align*}
    S_0 &:= C|F_0|^2, \\
    S_k &= 2C|F_k|^2, \quad k = 1, \ldots, \left\lfloor \frac{L}{2} \right\rfloor.
\end{align*}
The factor of 2 for $k > 0$ accounts for both negative and positive frequency contributions. This normalization ensures that Parseval's relation for energy is satisfied. Assuming $f_l$ are sampled values of a continuous function $f(\ell)$ over $0 < \ell < C$, the spacing of longitudinal samples is $C/L$. Thus:
\begin{equation*}
    \int_0^C |f(\ell)|^2 \, d\ell \approx \frac{C}{L} \sum_{l=0}^{L-1} |f_l|^2 = \sum_{k=0}^{\left\lfloor \frac{L}{2} \right\rfloor} S_k.
\end{equation*}

To obtain the final spectrum, the zonal spectra are averaged for latitude bands between $30^\circ < |\text{lat}| < 60^\circ$.

The global spherical harmonic analysis (GSHA)\cite{bonev2023spherical} reduces data to spherical harmonic coefficients $C_{lm}$ and $S_{lm}$ using:
\begin{equation*}
    f(\theta, \lambda) = \sum_{l=0}^\infty \sum_{m=-l}^l Y_l^m(\theta, \lambda) f_l^m,
\end{equation*}
where $Y_l^m(\theta, \lambda)$ are the spherical harmonics defined as:
\begin{equation*}
    Y_l^m(\theta, \lambda) = \sqrt{\frac{2l+1}{4\pi} \frac{(l-m)!}{(l+m)!}} P_l^m(\cos \theta) e^{im\lambda},
\end{equation*}
with $P_l^m(\cos \theta)$ being the normalized associated Legendre polynomials.

The spherical harmonic transform (SHT) projects a signal $f(\theta, \lambda)$ onto the spherical harmonic basis:
\begin{equation*}
    f_l^m = \int_{S^2} Y_l^m(\theta, \lambda)^* f(\theta, \lambda) \, d\mu(\theta, \lambda),
\end{equation*}
where $d\mu(\theta, \lambda)$ represents the measure $\sin \theta \, d\theta \, d\lambda$ on the sphere.

To approximate $f_l^m$ for discrete data, Gaussian quadrature is applied in the $\cos \theta$ domain:
\begin{equation*}
    f_l^m \approx \sum_{j=1}^{N_\theta} \sum_{k=1}^{N_\lambda} f(\theta_j, \lambda_k) Y_l^m(\theta_j, \lambda_k) w_j,
\end{equation*}
where $\theta_j$ and $w_j$ are the quadrature nodes and weights, and $\lambda_k$ represents uniform sampling in longitude.

\subsection{Kolmogorov-Smirnov test}\label{KS_test}
The Kolmogorov-Smirnov test (KS test) \cite{massey1951kolmogorov} is a widely used statistical method for comparing the empirical cumulative distribution function (CDF) of a sample dataset with either a reference probability distribution or another sample dataset. This test is particularly effective for evaluating whether two datasets originate from the same underlying distribution or if significant differences exist between them.

The KS test quantifies the maximum deviation between the two cumulative distribution functions. This deviation, represented by the KS statistic (D), measures the largest vertical distance between the empirical CDF of the sample and the theoretical CDF of the reference distribution. In cases where two sample datasets are compared, the KS statistic reflects the maximum difference between their respective empirical CDFs.

To determine the statistical significance of the observed KS statistic, it is compared to critical values derived from the Kolmogorov-Smirnov distribution. These critical values are influenced by the sample size and the significance level chosen for the test, providing a threshold for assessing whether the observed differences are statistically significant or attributable to random variation. The KS test is non-parametric, making it a versatile tool applicable across a wide range of distributions without requiring specific parametric assumptions.

\subsection{Derived variables}\label{Derived_variables}

We calculate variables that can be derived from geopotential, temperature, \( u \) component of wind, \( v \) component of wind, and specific humidity to better analyze and understand the inter-variable dependency of ML weather forecasts and climate projections.

\begin{enumerate}
    \item \textbf{Wind speed} is given by
    \[
    \sqrt{u^2 + v^2},
    \]
    where \( u \) and \( v \) denote \( u \)-component of wind velocity (zonal) and \( v \)-component of wind velocity (meridional).

    \item \textbf{The mass streamfunction} (\( \psi \)) is computed using the following formula:
    \[
    \psi(\phi, p) = \frac{2 \pi a \cos\phi}{g} \int_{p_{\text{top}}}^{p} v(\phi, p') \, dp',
    \]
    where \( \psi \) is the mass streamfunction (kg/s), \( g = 9.81 \, \text{m/s}^2 \) is the gravitational acceleration, \( a = 6371 \, \text{km} \) is the Earth's radius, \( \phi \) is the latitude (degrees), \( v(\phi, p') \) is the meridional wind (m/s), \( p \) is the pressure (Pa), \( p_{\text{top}} \) is the pressure at the top of the atmosphere.

    \item \textbf{Geostrophic wind} is a horizontal vector given by
    \[
    \frac{1}{2\Omega \sin \phi} \mathbf{\hat{k}} \times \nabla_p \Phi = \frac{1}{2\Omega \sin \phi} \left[ -\partial_y \Phi, \partial_x \Phi \right],
    \]
    where \( \Omega \) is the rotational speed of the Earth, \( \phi \) is latitude in radians, \( \nabla_p \) is the gradient on constant pressure levels, and \( \Phi \) is geopotential.
    
    \item \textbf{Ageostrophic wind} is the horizontal wind vector minus geostrophic wind \cite{bonavita2024some}.
    
    \item \textbf{Relative humidity} (\( RH \)) is calculated as:
    \[
    RH = \frac{e}{e_s} \times 100,
    \]
    where \( e \) is the actual vapor pressure (Pa), \( e_s \) is the saturation vapor pressure (Pa), which depends on temperature \( T \) and can be computed using the Clausius-Clapeyron relation.

    \item \textbf{Dew point temperature} (\( T_d \)) is estimated using:
    \[
    T_d = \frac{243.5 \, \ln(e/6.112)}{17.67 - \ln(e/6.112)},
    \]
    where \( T_d \) is the dew point temperature (°C), \( e \) is the actual vapor pressure (hPa).

    \item \textbf{Precipitable Water} (\( PW \)) is calculated using the vertical integral of specific humidity:
    \[
    PW = \frac{1}{g} \int_{p_{\text{top}}}^{p_{\text{surf}}} q \, dp,
    \]
    where \( PW \) is the precipitable water (kg/m²), \( g = 9.81 \, \text{m/s}^2 \) is the gravitational acceleration, \( q \) is the specific humidity (kg/kg), \( p_{\text{surf}} \) is the pressure at the surface (Pa), \( p_{\text{top}} \) is the pressure at the top of the atmosphere (Pa).
    
    In discrete form, \( PW \) is computed as:
    \[
    PW = \frac{1}{g} \sum_{i=1}^{N-1} \frac{q_i + q_{i+1}}{2} (p_{i+1} - p_i),
    \]
    where \( N \) is the number of pressure levels, \( q_i \) is specific humidity at level \( i \), \( p_i \) is the pressure at level \( i \).
    
    If there are NaN values in \( q \), we perform interpolation in the log-pressure coordinate ensuring physically consistent values. The integral result is divided by gravitational acceleration \( g \) to obtain precipitable water in \( kg/m^2 \).

\end{enumerate}

\subsection{Extreme events detection}\label{Extreme_events_detection}

\subsubsection{Tropical cyclones tracking}\label{TC_track_method}

A common method for assessing a cyclone trajectory involves initializing a cyclone tracker based on the observed cyclone initiation (usually the minimum of local mean sea leavel pressure) and continuing the tracking process until the cyclone dissipates. However, this approach has notable limitations, particularly in evaluating the accuracy of cyclone genesis and cyclone dissipation predictions. Furthermore, it cannot be directly applied to ensemble forecasts due to variations in cyclone lifetimes across ensemble members.

To address these challenges, we utilized the open-source \textit{TempestExtremes} cyclone tracker \cite{ullrich2021tempestextremes}. A resolution of 1° (approximately 111 km at the equator) was chosen as it closely aligns with the 120 km radius often used to define cyclone strike probabilities. For verification, cyclone trackers were applied to the GAP predictions or emulations and ERA5 datasets.
.

\textit{TempestExtremes} operates in two primary stages: Stage 1 include the detection of possible candidates. This stage identifies potential tropical cyclones based on minima in mean sea level pressure (MSL) co-located with upper-level warm cores. Candidates are firstly defined as local minima in MSL. Any candidate within 6° of a stronger MSL minimum is excluded. Each MSL minimum must be enclosed by a closed contour with at least 200 hPa stronger pressure than the minimum, contained within 5.5° of the MSL minimum. Then candidates must exhibit a warm-core structure, characterized by maxima in the geopotential thickness field (500 hPa to 300 hPa) ranging between 2500–2300 meters. The maxima must also be enclosed by a closed contour, with a thickness at least $58.8 \, \mathrm{m}^2\mathrm{s}^{-2}$ below the maximum, and confined within 6.5° of the geopotential thickness maximum.

The second stage is connecting candidate cyclones across time steps to form trajectories. Candidates must remain within 8° great-circle distance between consecutive time steps. Then trajectories can bridge a maximum of 24 hours between consecutive candidates. Gaps exceeding this threshold result in trajectory termination and cyclones must persist for at least 54 hours to qualify as tropical cyclones. Lastly candidates must meet thresholds for wind speed ($\geq 10 \, \mathrm{m/s}$), elevation ($< 150 \, \mathrm{m}$), and latitude (between $-50^\circ$ and $50^\circ$).

%These adjustments were carefully calibrated through visual inspection to strike a balance: a smaller stitch range risked prematurely terminating fast-moving cyclones, while a larger range could erroneously link separate storms. Although rare, the increased stitch range occasionally caused nearby but distinct storms to be incorrectly connected, but this did not introduce model-specific biases.

%All other \textit{TempestExtremes} hyperparameters were kept at their default values, and these adjustments were uniformly applied across all models and datasets.

\subsubsection{Blocking tracking}\label{Block_track_method}

Atmospheric blocking events, characterized by the disruption of the normal westerly flow, are associated with extreme weather phenomena such as heat waves, cold spells, flooding, and drought \cite{lupo2021atmospheric}. We also use \textit{TempestExtremes} to assess atmospheric blocking frequency. It involves initializing a blocking detection algorithm based on observed geopotential height anomalies and continuing the process to identify blocking events across spatial and temporal domains. \textit{TempestExtremes} detects and characterizes atmospheric blocking events using the modified Dole and Gordon algorithm \cite{dole1983persistent}. This algorithm identifies blocking events based on anomalously high values of geopotential height at 500 hPa (Z500), incorporating thresholds that account for climatological and seasonal variability.

The first step involves constructing a climatology of the Z500 field and determining a threshold for blocking detection. Following \cite{pinheiro2019atmospheric}, the threshold is defined as the daily mean Z500 value plus the greater of 100 m or 1.5 times the daily standard deviation of Z500. This threshold accounts for geographical and seasonal variations. Fourier smoothing is then applied to reduce noise in the daily data when calculating climatology.

The standard deviation of the Z500 field is then calculated. This results in a 365-day threshold field, which captures the geographical and seasonal variability of Z500. Blocking events are identified as contiguous regions where Z500 exceeds the threshold. These regions must meet specific spatial criteria, including latitudinal bounds and a minimum area of $10^6$ km$^2$. To qualify as a blocking event, regions must persist for at least 5 days. We connect blocking features across time steps, applying temporal persistence and overlap criteria. Finally, a seasonal climatology of blocking frequency is constructed. This procedure generates a comprehensive climatology of atmospheric blocking events, facilitating studies of their spatial and temporal distributions.

\subsection{Climate variability assessment}\label{Climate_variability_evaluation}

\subsubsection{Arctic Oscillation (AO)}
The Arctic Oscillation (AO) is a dominant mode of atmospheric variability in the Northern Hemisphere \cite{thompson1998arctic, thompson2000annular}. We identify and analyze the AO following the methodology of \cite{thompson2000annular}: we compute the leading Empirical Orthogonal Function (EOF) of the monthly mean sea level pressure (MSLP) anomalies north of 20°N. The spatial pattern is normalized to unit variance, and the associated principal component time series becomes the AO index. The spatial patterns are visualized as regression maps of MSLP anomalies onto the standardized AO index.

This analysis captures the characteristic dipole structure of the AO, with opposite-signed pressure anomalies between the Arctic and mid-latitudes. The EOF analysis is performed using singular value decomposition (SVD) to identify the dominant spatial patterns and their temporal evolution.

\subsubsection{Southern Oscillation Index (SOI)}
The Southern Oscillation Index (SOI) quantifies ENSO variability by measuring the normalized pressure difference between Tahiti and Darwin, Australia \cite{trenberth1984signal, ropelewski1987global}. We calculate the SOI following standard methodology \cite{trenberth1984signal}:

\begin{equation*}
\text{SOI} = 10 \times \frac{P_{\text{diff}} - \overline{P_{\text{diff}}}}{\sigma_{P_{\text{diff}}}}
\end{equation*}

where $P_{\text{diff}}$ is the difference between the standardized sea level pressure at Tahiti (17.5°S, 149.6°W) and Darwin (12.4°S, 130.9°E), $\overline{P_{\text{diff}}}$ is the long-term mean of this difference, $\sigma_{P_{\text{diff}}}$ is the standard deviation of this difference

Negative SOI values correspond to El Niño conditions (warmer eastern Pacific), while positive values indicate La Niña conditions (cooler eastern Pacific). The factor of 10 is applied by convention to scale the index to typically range between -35 and +35 \cite{trenberth1997definition}.

\clearpage

\section{Supplementary results}\label{Appendix_metrics}

In this section, we provide a comprehensive evaluation of GAP, highlighting its performance across all time scales in a range of critical metrics. The analysis encompasses climatology statistics, power spectrum characteristics, assimilation accuracy, weather forecast skill, seasonal prediction and climate projection performance. GAP demonstrates robust capabilities in simulating large-scale atmospheric dynamics, preserving spatio-temporal variability, providing competitive accuracy and meaningful uncertainty quantification.

The climatology evaluation underscores GAP's ability to capture key atmospheric features such as planetary-scale wave structures, meridional gradients, and dominant climate modes. Power spectrum analysis reveals that GAP maintains physically consistent scaling behaviors across scales, aligning closely with observational datasets. In data assimilation experiments, GAP excels in reducing ensemble variance and quantifying uncertainty, ensuring reliable state estimates even in data-sparse regions.

Forecast evaluation further highlights GAP's superiority in mid- to long-range weather prediction. Compared to state-of-the-art physical and machine learning models, GAP achieves competitive even higher skill scores for critical fields like geopotential height at 500 hPa (Z500) and demonstrates promising performance for extended lead times. Additionally, GAP effectively captures seasonal cycles and long-term variability in free-run simulations, validating its potential and applicability for seasonal and climate-scale modeling. These findings illustrate GAP's versatility and reliability for operational forecasting and climate research.

\subsection{Climatology statistics}

\subsubsection{Relative RMSE}

At individual grid scale, we first examine basic statistical measures (mean, variance, minimum, and maximum) across all variables and pressure levels to quantify GAP's fidelity in reproducing local climatological distributions. We compute these measures for both the reanalysis data and GAP-generated samples, then calculate their relative differences to assess model performance. The spatially averaged relative differences (SI Fig.~\ref{Climatology_suppli_relative_rmse}) reveal remarkable agreement between GAP and the reanalysis across the entire atmospheric domain, with typical deviations below 10\% for most variables and metrics. This close correspondence extends from surface variables through the troposphere to upper-level fields, demonstrating GAP's ability to capture the statistical properties of the atmosphere at point-scale resolution. Particularly strong agreement is observed for the mean and variance of temperature and geopotential height fields, while slightly larger deviations appear in moisture-related variables where relative humidity is naturally low and more variable.

\begin{figure}[h]
\centerline{\includegraphics[width=\linewidth]{suppli_fig/Climatology_suppli_relative_rmse.pdf}}
\caption{Relative error of statistical features across various pressure levels and variables (z: geopotential height, q: specific humidity, t: temperature, u: u-component of wind, v: v-component of wind)}\label{Climatology_suppli_relative_rmse}. 
\end{figure}

\subsubsection{Spatial distribution}

The spatially averaged field for geopotential height at 500 hPa (SI Fig.~\ref{fig_Climatology_z_suppli_1}) reveals a high level of agreement across multiple statistical measures. In the first two rows of panels (a--j) in Fig. \ref{fig_Climatology_z_suppli_1}, the analysis demonstrates that GAP successfully reproduces key atmospheric circulation features, including planetary-scale wave structures and meridional geopotential height gradients. In particular, the model captures dominant climate modes in the mid- to high-latitudes of the Northern Hemisphere, such as the North Atlantic Oscillation and the Arctic Oscillation, while also accurately depicting the subtropical high-pressure systems in low-latitude regions. This ability highlights the model's skill in simulating dynamic processes associated with the 500 hPa height field.

\begin{figure}[h]
\centering
\centerline{\includegraphics[width=\linewidth]{suppli_fig/Climatology_statistic_z_suppli.jpg}}
\caption{Climatology statistics of geopotential height at 500 hpa: mean field (first column), variance field (second column), minimum field (third column), maximum field (fourth column).}\label{fig_Climatology_z_suppli_1}
\end{figure}

Assessment of the spatially averaged relative humidity field (SI Fig.~\ref{fig_Climatology_q_suppli_1}) further validates GAP's effectiveness in simulating moisture distribution. Specifically, in tropical regions, the model accurately captures seasonal humidity variations and the strong moisture bands associated with the Intertropical Convergence Zone (ITCZ). In mid- to high-latitude regions, GAP effectively simulates the orographic dependence of humidity, such as enhanced moisture on the windward sides of the Tibetan Plateau and the Rocky Mountains. Additionally, the analysis reveals the model's capability to represent contrasts between arid regions (e.g., the Sahara Desert) and humid zones (e.g., the Amazon Rainforest), demonstrating its robustness in reproducing hydrological cycle processes.

\begin{figure}[h]
\centering
\centerline{\includegraphics[width=\linewidth]{suppli_fig/Climatology_statistic_q_suppli.jpg}}
\caption{Climatology statistics of specific humidity at 500 hpa: mean field (first column), variance field (second column), minimum field (third column), maximum field (fourth column).}\label{fig_Climatology_q_suppli_1}
\end{figure}

The statistical analysis of the 500 hPa temperature field shows that GAP accurately captures key climatological features, including the polar cold pools and the warm air masses over lower latitudes (SI Fig.~\ref{fig_Climatology_t_suppli_1}). In the latitudinal profile, the model successfully simulates the temperature gradient with height and latitude, while also capturing the distinctive thermal stratification of the tropical tropopause layer. Notably, the model excels in representing temperature contrasts between land and ocean, such as those observed over the North American continent and adjacent seas. Furthermore, the model's ability to replicate seasonal temperature variations, such as tropical warming during summer and polar cooling during winter, underscores its reliability in simulating temperature fields.

\begin{figure}[h]
\centering
\centerline{\includegraphics[width=\linewidth]{suppli_fig/Climatology_statistic_t_suppli.jpg}}
\caption{Climatology statistics of temperature at 500 hpa: mean field (first column), variance field (second column), minimum field (third column), maximum field (fourth column).}\label{fig_Climatology_t_suppli_1}
\end{figure}

The spatially averaged relative difference for the zonal wind at 500 hPa indicates that GAP effectively captures the planetary-scale jet streams and the low-latitude easterly wind patterns (SI Fig.~\ref{fig_Climatology_u_suppli_1}). The model accurately reproduces the core intensity and position of the mid-latitude westerly jet in the Northern Hemisphere, as well as the subtropical jet in the Southern Hemisphere. Furthermore, the model captures fine-scale variations in wind speed near complex terrains, such as the windward and leeward sides of the Andes and the Himalayas. This strong agreement with observed zonal wind patterns reflects the model's capability to simulate the dynamic processes governing large-scale wind fields.

\begin{figure}[h]
\centering
\centerline{\includegraphics[width=\linewidth]{suppli_fig/Climatology_statistic_u_suppli.jpg}}
\caption{Climatology statistics of u component of wind at 500 hpa: mean field (first column), variance field (second column), minimum field (third column), maximum field (fourth column).}\label{fig_Climatology_u_suppli_1}
\end{figure}

The analysis of meridional wind at 500 hPa (SI Fig.~\ref{fig_Climatology_v_suppli_1}) highlights DERA's precision in capturing interactions between zonal and meridional flows. The results show that the model performs exceptionally well in simulating the transition of meridional winds in monsoon regions, particularly for the Asian summer monsoon and the African monsoon. Additionally, GAP reproduces the convergence of airflows within the subtropical convergence zone and the strong meridional wind components within polar vortices. In the Southern Hemisphere, the model captures seasonal changes in meridional wind intensity over oceanic regions, such as the strengthening of southerly winds over the Southern Ocean. These results demonstrate the model's competence in simulating coupled dynamical and thermal processes in the wind fields.

\begin{figure}[h]
\centering
\centerline{\includegraphics[width=\linewidth]{suppli_fig/Climatology_statistic_v_suppli.jpg}}
\caption{Climatology statistics of v component of wind at 500 hpa: mean field (first column), variance field (second column), minimum field (third column), maximum field (fourth column).}\label{fig_Climatology_v_suppli_1}
\end{figure}

\subsubsection{Power spectra analysis}

To assess the spatial covariability and consistency of individual variables, we performed power spectrum analysis. SI Figs.~\ref{fig_psd_suppli_1} and ~\ref{fig_psd_suppli_2} show the power spectra of atmospheric variables at all pressure levels. These figures illustrate that the GAP model generates realistic and physically consistent meteorological fields for multiple atmospheric variables across different altitudes. The power spectral densities (PSDs) of various variables exhibit close alignment with observational data and demonstrate the preservation of characteristic atmospheric scaling behavior, particularly at large scales. While large-scale variability is well-represented, minor discrepancies are noted at smaller scales, particularly for variables such as geopotential height at higher altitudes. These discrepancies, however, do not undermine the overall physical consistency of the generated fields.

\begin{figure}[h]
\centering
\centerline{\includegraphics[width=\linewidth]{suppli_fig/PSD_suppli_1.pdf}}
\caption{Power spectral density (PSD) maps for upper air atmospheric variables (temperature, specific humidity, geopotential height, wind velocity) at different pressure levels (from 40 hpa to 400 hpa), using ERA5 random selected fields and GAP generated fields}\label{fig_psd_suppli_1}
\end{figure}

\begin{figure}[h]
\centering
\centerline{\includegraphics[width=\linewidth]{suppli_fig/PSD_suppli_2.pdf}}
\caption{Power spectral density (PSD) maps for surface atmospheric variables (temperature at 2m, mean sea level pressure and wind velocity at 10m) and upper air atmospheric variables (temperature, specific humidity, geopotential height, wind velocity) at different pressure levels (from 500 hpa to 1000 hpa), using ERA5 random selected fields and GAP generated fields}\label{fig_psd_suppli_2}
\end{figure}

These highlight the results of power spectrum analysis. The PSDs confirm the GAP model’s ability to preserve characteristic atmospheric scaling behavior across scales. We further examined the spatial covariability of referential and generated distributions using field-scale statistics. The averaged power spectrum density for the considered referential and generated data samples follows a similar power-law scaling, demonstrating that the GAP model effectively reproduces spatial variability across scales. These analyses underscore the capability of the GAP model to generate meteorological fields that are not only visually and physically plausible but also statistically consistent with observational datasets like ERA5. The ability to replicate large-scale atmospheric dynamics and spatial variability across scales highlights the model’s potential for various meteorological and climatological applications (i.e. realistic weather ensemble forecast and climate emulations).

\clearpage

\subsection{Assimilation evaluation}

Fig.~\ref{fig_DA_OSSE_V1} presents a case study of assimilation within a specific time window, from February 14 to March 12, 2022. This detailed analysis highlights how the ensemble evolves through the assimilation process, progressively reducing both the forecast error and ensemble spread as observations are incorporated.

\begin{figure}[h]
\centering
\centerline{\includegraphics[width=\linewidth]{suppli_fig/DA_OSSE_suppli_V1.jpg}}
\caption{A sequential assimilation case across the assimilation window (UTC 12:00, 24 February 2022 to UTC 12:00, 3 March 2022). The first row shows the atmospheric circulation from ERA5, while the second row displays the IFS t0 mean. The third and sixth rows present GAP assimilation results generated from operational observations and a perfect grid point (OSSE), respectively. The subsequent rows illustrate the standard deviation and error of the GAP assimilation.}\label{fig_DA_OSSE_V1}
\end{figure}

The assimilation process begins with a cold start, where ensemble members are initialized to agree with the available observations. GAP then propagates these members forward using its forecasting model, combining them with new incoming observations to iteratively update the ensemble. The assimilation reduces ensemble variance, particularly in regions close to observation points, while maintaining meaningful uncertainty estimates in data-sparse areas. This highlights the model's capability to integrate climatological priors with partial observations to produce probabilistic estimates of global atmospheric patterns.

The assimilation experiments utilize operational observations from approximately 100 radiosonde and pilot balloon stations under the Integrated Global Radiosonde Archive (IGRA). These observations provide pressure, temperature, geopotential height, humidity, and wind data at standard and variable pressure levels, updated every six hours with occasional gaps. Supplementary surface observations from the Integrated Surface Database are also incorporated, offering additional information such as surface pressure, temperature, and wind speed.

To evaluate the impact of observational quality and layout, we also conduct experiments with "perfect observations" derived from ERA5 at corresponding locations. This setup isolates observational uncertainty, allowing for a detailed assessment of the influence of observation density and distribution on the assimilation results.

The results indicate that GAP’s assimilation process effectively balances the chaotic growth of forecast uncertainty with observational constraints. As the assimilation progresses, the ensemble accuracy improves, with the ensemble spread and error converging to a stable state. The assimilation results also show strong correlations between ensemble variance and absolute error, ensuring reliable uncertainty quantification. This feature is particularly valuable for identifying regions requiring targeted observations to reduce uncertainty further.

Additionally, GAP demonstrates meaningful performance under varying observational densities. With increasing observation numbers, the saturation point—where additional observations provide diminishing returns—is reached earlier. This behavior underscores GAP’s ability to efficiently leverage observational data for accurate and robust ensemble forecasting.

In summary, the assimilation experiments confirm GAP's capability to integrate operational observations and generate diverse, physically consistent ensemble forecasts. By effectively reducing uncertainty and maintaining realistic atmospheric fields, GAP provides a reliable framework for both weather forecasting and climate modeling applications.

%\clearpage

For both the operational observations and ERA5 OSSE cases, the initial ensemble variance begins at a specific value and decreases as more observational data are assimilated into the system. This decrease reflects the system’s ability to reduce uncertainty in state estimates with additional data. Notably, at each time step, the spatial distribution of ensemble variance typically increases with distance from observational points, as illustrated in Fig~\ref{fig_assimilation_distance}. This pattern aligns with expectations, as regions further from observations naturally have less direct information to constrain state estimates.

\begin{figure}[h]
\centering
\centerline{\includegraphics[width=\linewidth]{suppli_fig/Assimilation_distance_suppli.pdf}}
\caption{RMSE statistics (y-axis) at different distance levels through the assimilation window (error in deep colors and variance in shallow colors)}\label{fig_assimilation_distance}
\end{figure}

A particularly important aspect of this analysis is the strong correlation between the ensemble variance and the absolute error of the ensemble mean (Fig~\ref{fig_assimilation_distance} and Fig~\ref{fig_assimilation_sensitivity_suppli}). This correlation indicates that areas with higher estimation errors are consistently associated with higher uncertainty estimates. Such a relationship is critical for reliable forecasting, as it ensures that regions with large uncertainties are not erroneously assigned high confidence. This feature enables decision-makers to identify areas of high uncertainty and prioritize targeted observations to improve estimates in those regions.

Moreover, this strong correlation remains stable over assimilation time, neither increasing nor decreasing significantly. This consistency suggests that the system maintains a reliable relationship between uncertainty quantification and estimation accuracy, independent of assimilation progress. Supporting figures or quantitative metrics can provide further evidence for this observation. The meaningful uncertainty quantification provided by GAP assimilation is a key advantage. By offering accurate uncertainty estimates without imposing strong assumptions like Gaussianity, it enables more reliable forecasts and supports adaptive strategies such as targeted observations. This capability is particularly valuable for applications where forecast reliability and uncertainty assessment are critical.

\begin{figure}[h]
\centering
\centerline{\includegraphics[width=\linewidth]{suppli_fig/Assimilation_sensitivity_suppli.pdf}}
\caption{RMSE skill (y-axis) at different observation density levels through the assimilation window for GAP (shading for ensemble members and blue line for ensemble mean) and IFS HRES analysis (black lines), on z500, as a function of assimilation window (x-axis)}\label{fig_assimilation_sensitivity_suppli}
\end{figure}

As more observations become available, the saturation point is reached earlier, highlighting the interplay between chaotic dynamics and observational constraints (Fig ~\ref{fig_assimilation_sensitivity_suppli}). The saturation point in the assimilation process reflects the balance between the chaotic growth of state estimate uncertainty and the constraining influence of observations. As the number of observations increases, the assimilation system can achieve higher accuracy in fewer assimilation steps. For instance, with 1,000 observations, the system requires three assimilation steps to reach the accuracy of IFS analysis; with 3,000 observations, it requires only two steps; with 5,000 observations, the initial estimate itself becomes significantly more accurate; and with 10,000 observations, no further assimilation is necessary. This illustrates the diminishing returns of adding more observations as the system becomes better constrained, reaching a point where additional data no longer improve the analysis significantly.

Importantly, the relationship between assimilation quality and the number of observations appears to follow a systematic pattern, potentially linear or exponential, which warrants further exploration. Understanding this relationship could offer insights into the efficiency of data usage in the assimilation process and help optimize observation network designs.

Additionally, as the number of observations increases, the impact of their spatial distribution on assimilation quality becomes less pronounced. When observations are sparse, their layout plays a critical role in determining which regions of the state space are well-constrained. However, as observations become denser, the system gains sufficient information to reduce dependence on specific layouts. This finding suggests that while careful observation placement is crucial for sparse networks, its importance diminishes with higher observation density. The saturation behavior of GAP assimilation underscores the dynamic interplay between observational constraints and the inherent chaotic nature of the system. By systematically analyzing how the saturation point shifts with varying observation numbers, we can better understand the trade-offs in observation network design and assimilation strategy, optimizing for both accuracy and efficiency.

We also provide an example of vertical profiles of temperature and dew point temperature from the assimilation field, demonstrating GAP's capability to capture the vertical structure accurately.

\begin{figure}[h]
\centering
\centerline{\includegraphics[width=0.6\linewidth]{suppli_fig/Assimilation_sounding_profile_suppli.pdf}}
\caption{Assimilation profile for selectd grid. Red line and shading show temperature profile and mean temperature profile. Green line and shading show dew point temperature profile and mean dew point temperature profile}\label{fig_assimilation_sounding_profile}
\end{figure}

In this example, the profiles are taken at a location 500 km away from the nearest observation point, highlighting the system's ability to estimate conditions in regions with limited observational constraints. The vertical profiles show that GAP assimilation faithfully reproduces the true vertical structure of both temperature and dew point temperature. This result underscores the robustness of the assimilation system in extrapolating information from observations to unobserved areas, even at significant distances.

Furthermore, GAP provides reasonable uncertainty estimates along the vertical profiles. The ensemble variance reflects the varying levels of confidence in the state estimates at different atmospheric layers. Notably, the uncertainty estimates tend to be larger at layers where observational constraints are weaker or where atmospheric variability is higher, such as near the tropopause or within moisture-rich layers. This behavior aligns with physical expectations, providing confidence in the system's ability to quantify uncertainty meaningfully.

The accurate representation and the associated uncertainty estimates of initial states are particularly valuable for atmospheric applications. Reliable assimilation is essential for tasks such as weather prediction, modeling, and process studies. Moreover, the uncertainty estimates offer an additional layer of information, allowing users to assess the reliability of the assimilation results and potentially target observations in regions of higher uncertainty to improve forecasts further. This example illustrates GAP's strengths in accurately capturing dynamics and providing meaningful uncertainty quantification, even in data-sparse regions. These capabilities enhance the system's utility for a wide range of atmospheric science applications for both operational and research purposes.

\subsection{Ensemble forecast of extreme events}\label{ensemble_forecast_of_extreme_events}

SI Fig.~\ref{fig_TC_ENS_case} illustrates the full set of 50 ensemble forecast samples generated by GAP for Typhoon INFA, shortly before its heavy rainfall impact in China on May 27, 2023. These forecasts demonstrate GAP's capability to capture the extreme atmospheric features associated with tropical cyclones, including intense wind speeds, low central pressures, and the characteristic spiral structure of a typhoon. Moreover, the ensemble framework highlights the inherent uncertainty in the typhoon’s trajectory, particularly regarding the landfall location—an aspect that deterministic forecasts often struggle to represent adequately.

\begin{figure}[h]
\centering
\centerline{\includegraphics[width=0.8\linewidth]{suppli_fig/TC_ENS_case_suppli_V1.jpg}}
\caption{A 3-day ensemble forecast case of typhoon In-fa. The lead time is 3 day. The geopotential height (contour), wind speed (color) and wind vector at the 500 hPa pressure level is presented. The first row displays ERA5 and the GAP ensemble mean, while the subsequent rows depict the 50 ensemble members.}\label{fig_TC_ENS_case}
\end{figure}

One notable characteristic of GAP's ensemble forecasts is their ability to generate high-fidelity samples that closely resemble the observed fields. This contrasts with the ensemble mean, which appears smoother and loses high-frequency spectral components. Such smoothing is common in ensemble means because they average out the variability across ensemble members. GAP's individual ensemble members, however, retain the fine-scale structures and extreme features critical for understanding and predicting severe weather events.

%This behavior is highlighted in Fig.~\ref{fig_TC_ENS_case}, where the spherical harmonic power spectra of GAP’s ensemble samples align closely with the ERA5 ground truth, demonstrating the model's capability to produce realistic samples that reflect the predictive forecast distribution.

%A comparison with machine learning deterministic models, such as Pangu, reveals an important distinction.

MSE-trained models like Pangu tend to produce forecasts that closely resemble the ensemble mean. While this approach reduces pointwise errors, it often sacrifices the representation of extremes and fails to account for the full distribution of possible outcomes. In contrast, GAP leverages its probabilistic framework to generate diverse and realistic ensemble members that better capture uncertainty and extreme weather events.

%Another critical advantage of GAP's ensemble approach is evident when computing nonlinear derived quantities, such as wind speed. Since wind speed is derived as the magnitude of the wind vector, it is a nonlinear function of the zonal (u) and meridional (v) wind components. Calculating wind speed directly from the ensemble mean of u and v can introduce biases, as the nonlinear operation does not commute with averaging. GAP avoids this issue by computing nonlinear functions at the sample level and then aggregating the results, thereby minimizing biases in derived quantities. As demonstrated, GAP exhibits minimal bias in wind speed predictions, while models like Pangu show significant negative biases due to their deterministic framework.

GAP's ensemble forecasts for Typhoon INFA showcase its strengths in capturing extreme weather features, representing uncertainty, and producing physically consistent samples that align with observed distributions. This capability not only enhances the reliability of severe weather forecasts but also provides a robust framework for applications requiring accurate representation of probabilistic outcomes and extreme events. By addressing limitations inherent in deterministic models, GAP represents a significant advancement in ensemble-based forecasting methodologies.

\clearpage

SI Fig ~\ref{fig_AR_ENS_case} showcases GAP's 10-day ensemble forecast of an atmospheric river (AR) event over the U.S. West Coast, a region frequently impacted by these intense moisture transport phenomena. Atmospheric rivers are narrow corridors of concentrated water vapor in the atmosphere that can lead to extreme precipitation and severe weather conditions, making their accurate prediction crucial for disaster preparedness and resource management.

\begin{figure}[h]
\centering
\centerline{\includegraphics[width=0.8\linewidth]{suppli_fig/AR_ENS_case_suppli_V1.jpg}}
\caption{A 10-day ensemble forecast case of the atmospheric river. The lead time is 10 day. The geopotential height (contour), specific humidity (color) and wind vector at the 700 hPa pressure level is presented. The first row displays ERA5 and the GAP ensemble mean, while the subsequent rows depict the 50 ensemble members.}\label{fig_AR_ENS_case}
\end{figure}

The figure highlights GAP's capability in capturing the formation, development, and progression of the atmospheric river. The model effectively resolves the 850 hPa geopotential height field, demonstrating strong alignment with the ERA5 ground truth. Key features such as the ridges and troughs that guide the AR's trajectory are well-represented, emphasizing GAP's skill in simulating the large-scale atmospheric dynamics that drive these events. Furthermore, GAP provides detailed forecasts of the specific humidity field, accurately depicting the moisture plume's intensity and spatial extent.

One of GAP's strengths lies in its ability to maintain coherent representations of the AR throughout the 10-day forecast period. Although some uncertainty is naturally present in long-range forecasts, GAP consistently captures the broad signals of the atmospheric river's evolution. Notably, the model's ensemble forecasts effectively convey the range of potential paths and intensities for the AR, offering valuable insights into forecast uncertainty. As the lead time decreases, GAP’s predictions become increasingly precise, narrowing the uncertainty in the AR's trajectory and better resolving the regions most likely to experience heavy precipitation.

The forecast progression also highlights GAP's utility in predicting the timing and spatial distribution of key features associated with atmospheric rivers, such as moisture convergence zones and precipitation bands. These aspects are critical for anticipating the impacts of AR events, including flash flooding, landslides, and disruptions to water resource management.

This case study shows GAP's ability to forecast extreme weather events, particularly those characterized by complex interactions between large-scale atmospheric patterns and localized moisture transport. By accurately capturing both the deterministic and probabilistic aspects of atmospheric rivers, GAP demonstrates its value as a powerful tool for operational forecasting and risk assessment in the context of high-impact weather events.

\clearpage

SI Fig \ref{fig_HW_ENS_case} presents GAP's three-week ensemble forecast of an extreme heatwave that affected parts of Europe during the summer of 2021, bringing record-breaking temperatures and widespread impacts. Heatwaves, characterized by prolonged periods of abnormally high temperatures, pose significant challenges for forecasting due to their dependence on complex atmospheric dynamics and persistent large-scale patterns. This case study highlights GAP’s ability to predict such high-impact events with increasing precision over extended forecast horizons.

\begin{figure}[h]
\centering
\centerline{\includegraphics[width=0.8\linewidth]{suppli_fig/HW_ENS_case_suppli_V3.jpg}}
\caption{A 21-day ensemble forecast case of the heatweave. The lead time is 3-week. The geopotential height (contour), specific humidity (color) and wind vector at the 700 hPa pressure level is presented. The first row displays ERA5 and the GAP ensemble mean, while the subsequent rows depict the 50 ensemble members.}\label{fig_HW_ENS_case}
\end{figure}

GAP's forecasts effectively capture the evolution of the heatwave, from its early development to its peak intensity and eventual dissipation. In the forecasts from day 14 to day 21, GAP demonstrates strong alignment with ERA5 observations, accurately identifying the heatwave's core regions with extreme temperatures. The model successfully resolves the spatial extent of the heatwave, including its impact on Southern and Central Europe, where the most severe conditions were observed. This capability underscores GAP's skill in representing the large-scale atmospheric patterns, such as blocking highs, that contribute to the persistence and intensity of heatwave events.

While early forecasts exhibit some smoothing of temperature extremes, typical of ensemble mean predictions, GAP’s probabilistic framework captures the full range of possible outcomes. Ensemble members provide diverse scenarios for the heatwave's evolution, including variations in intensity, spatial extent, and timing. This allows for a comprehensive assessment of forecast uncertainty, crucial for long-range predictions where small initial condition differences can significantly affect outcomes. As the forecast lead time shortens, GAP’s predictions converge, with increased accuracy in pinpointing the regions of highest risk and better resolving localized temperature extremes.

Importantly, GAP’s ability to forecast the progression of the heatwave over multiple weeks demonstrates its value for long-range climate and weather prediction. The gradual refinement of the forecast reflects the model's capacity to incorporate updated information and improve predictions over time. By accurately predicting the spatial and temporal characteristics of heatwaves, GAP provides essential information for early warnings and risk mitigation, helping governments, industries, and communities prepare for the impacts of such extreme events.

This case highlights GAP's robustness in forecasting extended-duration, high-impact weather events. Its ability to capture the key features of an extreme heatwave in a three-week forecast horizon reinforces its potential as a critical tool for operational weather forecasting and climate risk assessment in an era of increasing weather extremes.

\clearpage

SI Fig ~\ref{fig_MJO_ENS_case} showcases GAP's 42-day ensemble forecast of the Madden-Julian Oscillation (MJO), a dominant mode of intraseasonal variability that significantly impacts tropical climates and global weather patterns. The MJO influences a wide range of phenomena, from seasonal precipitation patterns to the modulation of tropical cyclone activity, making accurate forecasts of its evolution critical for both operational and research applications.

\begin{figure}[h]
\centering
\centerline{\includegraphics[width=0.8\linewidth]{suppli_fig/MJO_ENS_case_suppli_V1.pdf}}
\caption{A 42-day ensemble forecast case of MJO. The lead time is 32 day. The wind anomaly (color) at the 200 hPa pressure level is presented. The first row displays ERA5 and the GAP ensemble mean, while the subsequent rows depict the 50 ensemble members.}\label{fig_MJO_ENS_case}
\end{figure}

GAP's forecast demonstrates strong performance in capturing the spatiotemporal evolution of the MJO signal over the 42-day period. The model successfully predicts the MJO’s phase propagation across the tropics, as well as its intensity, aligning closely with ERA5 observations. The characteristic eastward movement of enhanced and suppressed convection patterns, which define the MJO, is well-represented in GAP’s forecasts. This is particularly evident in the accurate depiction of convective anomalies over the Indian Ocean, Maritime Continent, and Pacific Ocean, key regions where the MJO exerts its most significant influence.

A notable strength of GAP is its ability to maintain forecast accuracy even at extended lead times. While long-range forecasts inherently involve increasing uncertainty, GAP effectively mitigates this by providing probabilistic ensemble predictions. These ensemble forecasts capture the range of potential outcomes for the MJO’s phase and intensity, offering valuable insights into forecast confidence. Despite the challenges associated with the MJO's complex dynamics and interaction with other atmospheric processes, GAP demonstrates minimal bias in its predictions, ensuring reliable guidance for extended-range forecasting.

The forecast progression also highlights GAP’s capability to predict the intensity of the MJO signal, which is crucial for understanding its downstream impacts. For example, stronger MJO phases often correlate with enhanced tropical cyclone activity and shifts in monsoonal rainfall patterns. GAP’s accurate intensity forecasts enable better preparation for these associated weather events, enhancing its utility for sectors like agriculture, water resource management, and disaster mitigation.

In summary, GAP’s 42-day forecast of the MJO underscores its potential as a robust tool for extended-range forecasting. By accurately capturing the MJO’s phase, intensity, and propagation, GAP provides critical information for understanding and predicting tropical climate variability. This capability not only supports operational forecasting but also contributes to advancing our knowledge of the complex interactions within the Earth’s climate system.

\clearpage

\subsection{Weather forecast accuracy and predictability}

ACC (anomaly correlation coefficient) is one of the most critical metrics for evaluating weather forecasting performance, particularly for mid-range forecasts. Here we provide a comprehensive comparison for both state-of-the-art physical and ML models: Pangu, GraphCast, NeuralGCM ensemble, and IFS ensemble (SI Fig \ref{fig_FC_ACC_suppli}). We also show the ensemble spread of GAP.

\begin{figure}[h]
\centering
\centerline{\includegraphics[width=1\linewidth]{suppli_fig/FC_ACC_suppli.pdf}}
\caption{A comprehensive comparison of anomaly correlation coefficients (ACC) with lead times extended to 28 days. The GAP ensemble is shaded, with the blue line representing the GAP ensemble mean.}\label{fig_FC_ACC_suppli}
\end{figure}

Our analysis reveals that GAP exhibits greater forecasting skill than determinstic ML models like Pangu and GraphCast when tested on 10-day forecasts at a horizontal resolution of 1.5 degree latitude-longitude. Figure \ref{fig_metrics} highlights GAP's superiority (blue line) over Pangu (orange line) and Graphcast (grey dotted line) in terms of ACC metrics, particularly for the geopotential height at 500 hPa (Z500). Z500, often referred to as the "headline" field in meteorology, is a critical parameter representing the synoptic-scale pressure distribution. Its importance lies in its strong correlation with large-scale atmospheric dynamics, making it a standard benchmark for assessing forecast skill \cite{rasp2020weatherbench}.

The results demonstrate that GAP consistently outperforms across all forecast lead times, with skill score improvements ranging from approximately 7\% to 14\%. These improvements are particularly notable at medium-range lead times, where the challenges of forecasting chaotic atmospheric dynamics are most pronounced. The superior performance of GAP in ACC indicates its enhanced capability to maintain coherence in atmospheric structures over extended periods, a critical aspect for both operational forecasting and potential extended prediction.

Furthermore, SI Fig. \ref{fig_FC_CRPS_suppli} compares the spatial CRPS of Z500 for 5-day, 10-day, and 15-day forecasts from GAP, IFS ensemble (IFS ens), and NeuralGCM ensemble (NeuralGCM ens). Overall, GAP, NeuralGCM ens, and IFS ens demonstrate similar spatial patterns of skill as measured by CRPS. However, GAP exhibits slightly lower spatial biases compared to ECMWF-ENS and NeuralGCM, with its biases also being more evenly distributed across regions. This suggests that GAP provides a more balanced representation of forecast accuracy across different geographical areas.

\begin{figure}[h]
\centering
\centerline{\includegraphics[width=1\linewidth]{suppli_fig/FC_CRPS_suppli.pdf}}
\caption{Maps of average CRPS for GAP, IFS ensemble and NeuralGCM ensemble for all forecasts in 2020. The lead times are 5 day, 10 day and 15 day.}\label{fig_FC_CRPS_suppli}
\end{figure}

In addition, we extended the forecast horizon for GAP to include 20-day and 25-day forecasts (Fig. \ref{fig_FC_CRPS_suppli_2}) and compared their spatial CRPS. Currently, equivalent forecasts for such extended lead times are unavailable from IFS ens and NeuralGCM ens due to limitations in their archived data. The results for GAP indicate promising performance in certain regions, particularly in the tropics, where it demonstrates consistent skill. This is noteworthy as tropical regions are known for their challenging predictability due to the dominance of small-scale and chaotic processes.

\begin{figure}[h]
\centering
\centerline{\includegraphics[width=0.7\linewidth]{suppli_fig/FC_CRPS_suppli_2.pdf}}
\caption{Maps of average CRPS for GAP for all forecasts in 2020. The lead times are extended for 20 day and 25 day.}\label{fig_FC_CRPS_suppli_2}
\end{figure}

The ability of GAP to provide skillful forecasts at 20-day and 25-day lead times opens up the potential for extended-range predictions at the subseasonal to seasonal (S2S) scale. This capability is critical for applications requiring longer-term planning, such as disaster preparedness, agriculture, and energy resource management. These findings highlight the adaptability and robustness of GAP in handling extended forecast horizons, offering a pathway for advancing operational capabilities in S2S prediction. In conclusion, GAP's improved ACC and CRPS scores across multiple variables and lead times underscore its advancement in weather scale. By demonstrating superior skill compared to Pangu and Graphcast, particularly in critical fields like Z500, GAP establishes itself as a powerful tool for accurate and reliable weather forecasting.

\subsection{Seasonal prediction}\label{SI_seasonalprediction}

To assess the seasonal forecasting skill of GAP, we compare its performance with SEAS5 (ECMWF’s operational seasonal forecasting system) \cite{johnson2019seas5}, as well as there additional baseline models: an SST anomaly persistence model and a free-run model, coupled seasonal prediction model from Canadian met office (CanCM4) and the GFDL physical model (Fig. \ref{fig_S2S_ACC_suppli}). These comparisons provide deeper insight into GAP’s predictive skill and its advantages over traditional and empirical forecasting approaches.

\begin{figure}[h]
\centering
\centerline{\includegraphics[width=0.8\linewidth]{suppli_fig/S2S_ACC_suppli.jpg}}
\caption{An inter-model comparison of Anomaly Correlation Coefficient (ACC) of monthly mean 2m temperature at lead time of 2-month, 3-month and 4-month. 4 models are included: GAP, GAP$_{\text{SAP}}$, SEAS5 and GFDL SPEAR.}\label{fig_S2S_ACC_suppli}
\end{figure}

Fig. \ref{fig_S2S_ACC_suppli} presents the seasonal prediction performance of GAP$_{\text{SAP}}$ compared with baseline model. GAP achieves higher accuracy in predicting the monthly mean near-surface temperature (T2m) at 2-month and 3-month lead times, maintaining comparable skill with SEAS5 at 4-month lead time. The anomaly correlation coefficient (ACC) spatial patterns of GAP closely resemble those of SEAS5, particularly in tropical regions, where its high predictive skill aligns with known seasonal climate drivers, such as ENSO-related teleconnections.

For SST anomaly persistence model, this simple baseline assumes that sea surface temperature anomalies persist unchanged throughout the forecast period, providing a reference for evaluating the added value of dynamic models. The SST persistence model demonstrates some predictive capability, particularly at shorter lead times, though its skill declines more rapidly than dynamical models at longer lead times.

Unlike GAP$_{\text{SAP}}$, the free-run model operates without external constraints, relying solely on its internal climate dynamics. As a result, its forecast skill degrades rapidly beyond 3 months, with ACC scores dropping significantly after this threshold. This highlights the importance of incorporating external constraints, such as SST forcing, in improving seasonal forecast skill.

The GFDL physical model, while capturing large-scale climate dynamics, exhibits lower accuracy than SEAS5 across most lead times, suggesting that additional constraints or bias correction may be needed to improve its performance. In contrast, GAP consistently outperforms GFDL, demonstrating the strength of its generative modeling approach in leveraging historical climate states for improved predictability.

Fig. \ref{fig_S2S_ACC_suppli} also presents an expanded inter-model comparison including additional baseline models. The CanCM4 model shows moderate skill with ACC values of 0.435, 0.344, and 0.311 at 2-, 3-, and 4-month lead times respectively, performing better than GAP but not reaching the skill levels of SEAS5 or GAP$_{\text{SAP}}$.

While GAP demonstrates strong predictive accuracy, some biases persist in land temperature forecasts. Despite this, GAP excels in predicting regional climate variations, particularly over Africa and South America, where it often outperforms both SEAS5 and the GFDL physical model. This suggests that GAP effectively captures regional-scale climate variability, making it a promising tool for improving seasonal forecasts in data-sparse regions.

By outperforming traditional physical models (GFDL, CanCM4) and empirical baselines (SST anomaly persistence, free-run models) in seasonal prediction, GAP proves to be a robust and reliable alternative for long-lead climate forecasting. Its ability to maintain high accuracy beyond 3-month lead times, while capturing key seasonal climate patterns, highlights its potential for probabilistic climate prediction, risk assessment, and improved operational forecasting.

\begin{figure}[h]
\centering
\centerline{\includegraphics[width=0.8\linewidth]{suppli_fig/S2S_CRPS_suppli.jpg}}
\caption{An inter-model comparison of Continuous Ranked Probability Score (CRPS) of monthly mean 2m temperature at lead time of 2-month, 3-month and 4-month. 3 models are included: GAP free run, GAP$_{\text{SAP}}$ and SEAS5.}\label{fig_S2S_CRPS_suppli}
\end{figure}

To further assess the probabilistic skill of GAP, we evaluate its performance using the Continuous Ranked Probability Score (CRPS), a widely used metric for probabilistic forecasting. Here, we compare GAP, GAP free-run, and SEAS5, focusing on their ability to provide calibrated and reliable seasonal forecasts (Fig. \ref{fig_S2S_CRPS_suppli}).

Fig. \ref{fig_S2S_CRPS_suppli} presents the CRPS scores for GAP, GAP free-run, and SEAS5 at different lead times. Lower CRPS values indicate better probabilistic calibration and overall forecast skill. At 1-month and 2-month lead times, GAP and SEAS5 exhibit similar CRPS scores, both outperforming the free-run model. This suggests that incorporating external constraints, such as prescribed SST forcing, significantly enhances probabilistic skill. At 3-month lead time, GAP maintains strong performance, with CRPS scores close to SEAS5 over oceanic regions. However, over land, GAP starts to show increasing biases, leading to a gradual decline in its CRPS score compared to SEAS5. At 4-month lead time and beyond, SEAS5 maintains a slight advantage over GAP in terms of probabilistic skill, particularly over land regions. The free-run GAP model, on the other hand, sees a rapid degradation in CRPS, highlighting the importance of external forcings for maintaining long-term forecast reliability. 

While GAP effectively captures large-scale climate patterns, an important limitation emerges at longer lead times (beyond 3 months), particularly over land regions. As shown in Fig. \ref{fig_S2S_CRPS_suppli}, GAP exhibits a systematic warm bias in some continental areas, likely due to the lack of additional land-atmosphere interactions and soil moisture constraints. This suggests that GAP’s reliance on SST as the primary external forcing may limit its skill over land at extended forecast horizons, where other factors such as soil moisture memory, vegetation feedbacks, and surface fluxes play a larger role.

GAP outperforms GAP free-run in CRPS scores at all lead times, demonstrating the importance of external forcing constraints in improving probabilistic calibration. GAP and SEAS5 exhibit comparable skill at short to medium lead times (1-2 months), particularly over oceanic regions. Beyond 3 months, GAP begins to show biases over land, leading to a decline in CRPS relative to SEAS5. The free-run GAP model rapidly loses skill beyond 2 months, reinforcing the need for additional constraints to maintain forecast accuracy.

While GAP offers competitive probabilistic forecasts and strong seasonal prediction skill, its performance over land at extended lead times (3+ months) remains an area for improvement. Future work could explore the integration of additional Earth system constraints, such as soil moisture anomalies and land-atmosphere coupling, to mitigate these biases. Despite these challenges, GAP remains a promising tool for seasonal forecasting, particularly in ocean-driven climate variability regimes, where it rivals operational models like SEAS5.

To further assess the relative probabilistic skill of GAP, we evaluate its Continuous Ranked Probability Skill Score (CRPSS), which measures improvement over a reference model. Here, SEAS5 serves as the benchmark, and we compare GAP and GAP free-run to determine how well they perform relative to this operational seasonal forecasting system (Fig. \ref{fig_S2S_CRPSS_suppli}).

\begin{figure}[h]
\centering
\centerline{\includegraphics[width=0.8\linewidth]{suppli_fig/S2S_CRPSS_suppli.jpg}}
\caption{An inter-model comparison of Continuous Ranked Probability Skill Score (CRPSS) of monthly mean 2m temperature at lead time of 2-month, 3-month and 4-month. 3 models are included: GAP free run, GAP$_{\text{SAP}}$ and SEAS5.}\label{fig_S2S_CRPSS_suppli}
\end{figure}

Fig. \ref{fig_S2S_CRPSS_suppli} resents the CRPSS scores for GAP and GAP free-run, using SEAS5 as the reference model. Higher CRPSS values indicate better probabilistic skill relative to SEAS5, while negative values indicate worse performance. GAP's performance over land declines beyond 3 months, leading to lower CRPSS scores relative to SEAS5. This suggests that while SST forcing provides strong constraints over the ocean, it is insufficient to fully capture land-atmosphere interactions, which play a dominant role in extended seasonal forecasts over continents. Missing constraints such as soil moisture variability, vegetation feedbacks, and surface fluxes may contribute to this performance gap.

At 3-month lead time, GAP’s CRPSS begins to decline over land, reflecting increasing biases in near-surface temperature forecasts. Beyond 3 months, GAP’s skill over land falls below SEAS5, indicating the need for additional land-atmosphere coupling constraints. GAP free-run consistently underperforms SEAS5, confirming the critical role of external forcings in seasonal forecasting.

The CRPSS results reaffirm the findings from CRPS evaluations, showing that GAP offers strong probabilistic skill in seasonal forecasting, particularly for ocean-driven variability. However, its performance over land at longer lead times remains a challenge, likely due to the absence of key land-atmosphere interactions.

\begin{figure}[h]
\centering
\centerline{\includegraphics[width=0.8\linewidth]{suppli_fig/S2S_z500_ACC_suppli.jpg}}
\caption{An inter-model comparison of ACC of monthly mean z500 at lead time of 2-month, 3-month and 4-month. 3 models are included: GAP, GAP$_{\text{SAP}}$ and SEAS5.}\label{fig_S2S_z500_CRPS_suppli}
\end{figure}

The comparison extends to 500hPa geopotential height (z500) predictions (Fig. \ref{fig_S2S_z500_CRPS_suppli}), where GAP$_{\text{SAP}}$ shows competitive performance with ACC values of 0.352, 0.365, and 0.279 for 2-, 3-, and 4-month leads. While SEAS5 maintains slightly higher ACC values (0.386, 0.368, 0.375), GAP$_{\text{SAP}}$'s skill remains robust, particularly in capturing large-scale atmospheric circulation patterns. The GAP free run shows notably lower skill, with ACC values of 0.257, 0.159, and 0.057 for 2-, 3-, and 4-month leads respectively, highlighting the crucial role of external forcing in maintaining prediction skill for upper-level atmospheric circulation.

\begin{figure}[h]
\centering
\centerline{\includegraphics[width=\linewidth]{suppli_fig/S2S_regional_PCC_suppli.pdf}}
\caption{Comparison of regional Pearson correlation coefficient (PCC) of monthly mean t2m at lead time of 3-month. 2 models are included: GAP$_{\text{SAP}}$ and SEAS5. 8 regions are included: North Atlantic, Indian Ocean, North Hemisphere Land, Africa, South America, North America, Eurasia and North Pacific.}\label{S2S_regional_PCC_suppli}
\end{figure}

The regional analysis (Fig. \ref{S2S_regional_PCC_suppli}) spanning 1991-2020 reveals distinct patterns in oceanic regions, with the Indian Ocean showing remarkably consistent prediction skill for both GAP$_{\text{SAP}}$ and SEAS5. PCC values frequently exceed 0.4 in this region, with GAP$_{\text{SAP}}$ demonstrating particularly strong performance post-2000. The North Atlantic and North Pacific exhibit higher variability, with GAP$_{\text{SAP}}$ achieving occasional peak performances exceeding 0.7 PCC, though skill in these basins shows pronounced interannual fluctuations. This enhanced predictability in ocean regions likely stems from strong ocean-atmosphere coupling mechanisms and the models' effective capture of major circulation patterns.
Continental regions display more diverse performance characteristics. South America stands out with consistently high PCC values above 0.5 for both models, with GAP$_{\text{SAP}}$ frequently matching or exceeding SEAS5's performance. This contrasts with more variable skill over North America and Eurasia, where both models show moderate performance with PCC values typically ranging from 0.2 to 0.4. Africa presents an interesting case where SEAS5 maintains relatively stable performance throughout the period, while GAP$_{\text{SAP}}$ shows strong early performance but increased variability in recent years, including some periods of negative correlation post-2010.
The Northern Hemisphere land regions collectively demonstrate a clear seasonal dependency in prediction skill, with both models showing reduced accuracy during transition seasons. This pattern is particularly pronounced in North America and Eurasia, where the models occasionally exhibit periods of negative correlation. The temporal evolution of skill varies significantly across regions, with some showing marked improvement in recent years (e.g., GAP$_{\text{SAP}}$'s performance in North America) while others maintain more consistent performance levels throughout the study period.
This comprehensive regional analysis underscores GAP$_{\text{SAP}}$'s competitive performance across diverse geographical domains, particularly excelling in regions dominated by strong ocean-atmosphere coupling. The model demonstrates robust skill in capturing both oceanic and continental climate variability, though with notable spatial and temporal variations that reflect the underlying complexity of regional climate systems and their predictability.

\newpage

\subsection{Climate projection}\label{climate_projection}

To evaluate GAP's ability to simulate historical temperature trends, we conducted AMIP-like simulations over a 40-year period (SI Fig \ref{fig_AMIP_40yr_t2m}). These simulations were compared against ERA5 observational data and included two configurations: one using prescribed t2m over ocean from ERA5 (refer to SAT), and another free-run experiment without any prescribed forcing. This experimental setup allowed us to assess GAP's performance under both constrained and unconstrained scenarios, providing insights into its capability to capture global climate variability and trends.

\begin{figure}[h]
\centering
\centerline{\includegraphics[width=0.9\linewidth]{suppli_fig/AMIP_40yr_t2m_suppli.pdf}}
\caption{Yearly global mean temperature for ERA5 (black), four GAP AMIP-like simulations with prescribed SST (grey lines), and one GAP free-run simulation (blue line). Monthly mean values from these experiments are shown in the lower panel.}\label{fig_AMIP_40yr_t2m}
\end{figure}

In the simulations where GAP was driven by ERA5 SATs, the model effectively reproduced the observed global warming trends over the 40-year period. The year-to-year temperature variations in these simulations exhibited a strong correlation with ERA5 data, highlighting GAP's ability to capture the influence of SST forcing on atmospheric temperature. Key features of the observed warming, including the spatial distribution of temperature anomalies and the pronounced warming over land and high latitudes, were accurately simulated. This demonstrates that GAP is capable of resolving the critical interactions between SST forcing and atmospheric processes that drive historical climate trends.

In the free-run experiment, which lacked any external forcing, GAP faithfully reproduced the annual cycle of surface air temperature (SAT) over the 40 years. However, as expected, the absence of external drivers such as increasing greenhouse gas concentrations resulted in no discernible global warming trend. The model's ability to maintain a realistic annual cycle and simulate internal variability without external constraints underscores its strong climatological priors and inherent dynamical consistency. This experiment highlights the role of external forcing in driving long-term climate trends, while also validating GAP's capacity to simulate baseline climatology.

To further analyze the simulations, we performed an empirical orthogonal function (EOF) analysis of SAT variability across the different experimental setups (SI Fig \ref{fig_AMIP_SST_EOF}). In the simulations with prescribed SST forcing, the first EOF mode closely matched that of ERA5, with the strongest variability located in the Niño regions. This alignment reflects GAP's ability to capture the dominant modes of climate variability, such as those associated with the El Niño-Southern Oscillation (ENSO). Additionally, the principal component (PC) amplitude time series for this mode showed high temporal consistency with ERA5, further validating GAP's ability to simulate interannual variability linked to SST anomalies.

\begin{figure}[h]
\centering
\centerline{\includegraphics[width=0.7\linewidth]{suppli_fig/AMIP_SST_EOF_suppli.jpg}}
\caption{EOF analysis of surface air temperature from ERA5, the GAP free-run experiment, and the GAP prescribed SST experiment. The first column displays the spatial fields of EOF mode 1, while the second column presents the amplitude of EOF mode 1.}\label{fig_AMIP_SST_EOF}
\end{figure}

In the free-run experiment, while the EOF structure differed due to the absence of external SST variability, the first mode still captured significant internal variability patterns, indicating that GAP accurately represents intrinsic atmospheric dynamics. These results emphasize the critical role of SST forcing in shaping observed climate variability while demonstrating GAP's robust handling of both externally forced and internally driven variability.

The combination of AMIP-like simulations and free-run experiments highlights GAP’s strong ability to simulate historical temperature trends and interannual variability. When driven by prescribed SSTs, GAP accurately reproduces observed warming patterns and climate fluctuations, underscoring its potential for studying atmospheric responses to external forcing. Additionally, EOF analysis confirms that GAP successfully captures dominant variability modes such as ENSO, further demonstrating its reliability for climate modeling.

To further evaluate GAP’s capability in climate projection, we conduct ensemble climate simulations using near-surface temperature over the ocean (t2m) from the Community Earth System Model version 2 (CESM2) as an additional constraint \cite{danabasoglu2020community}. This experiment allows us to assess how GAP responds to externally prescribed climate conditions and whether it can maintain physical consistency over extended timescales. The results demonstrate that GAP effectively reduces historical biases in key climate variables such as precipitable water, while preserving large-scale dynamical structures. Moreover, GAP exhibits possible generalization to future climate scenarios, accurately capturing major climate variability patterns and extreme events. However, there is a bias in temperature trend and air temperature which we will discuss later.

\begin{figure}[h]
\centering
\centerline{\includegraphics[width=0.8\linewidth]{suppli_fig/CESM_tem_vertical_history.jpg}}
\caption{History (1979-2014) JJA and DJF season zonal mean troposphere temperature from ERA5 and GAP.}\label{fig_CESM_t_vertical}
\end{figure}

Accurate representation of vertical temperature structure is critical for understanding atmospheric energy transport, convection, and climate feedback mechanisms. Figure~\ref{fig_CESM_t_vertical} demonstrates that GAP simulations closely align with CESM2 constraints. Unlike many machine learning models that exhibit temperature drift or physically implausible vertical gradients, GAP maintains consistent lapse rates and realistic temperature stratification across different atmospheric layers. This physical consistency ensures stable long-term projections that conform to established climate dynamics.

\begin{figure}[h]
\centering
\centerline{\includegraphics[width=0.8\linewidth]{suppli_fig/CESM_u_vertical_history.jpg}}
\caption{History (1979-2014) JJA and DJF season zonal mean wind from ERA5 and GAP.}\label{fig_CESM_u_vertical}
\end{figure}

\begin{figure}[h]
\centering
\centerline{\includegraphics[width=0.8\linewidth]{suppli_fig/CESM_future_JJA_tem_vertical_history.jpg}}
\caption{GAP future projections (2070-2100) under different scenarios (free run, SSP126, SSP370 and SSP585). Resoults show JJA season zonal mean troposphere temperature.}\label{fig_CESM_t_vertical_JJA_future}
\end{figure}

The vertical structure of wind fields is equally essential for simulating atmospheric circulation, storm development, and large-scale climate patterns. Figure~\ref{fig_CESM_u_vertical} reveals GAP's ability to reproduce complex zonal wind patterns with remarkable fidelity, including the strong westerly jets in the upper troposphere and stratosphere, alongside the weaker easterly flows in the lower atmosphere. When compared to CESM2, GAP preserves crucial dynamical features without introducing the over-smoothing or artificial distortions commonly observed in purely data-driven approaches.

To further assess GAP’s ability to generalize beyond historical conditions, we analyze its vertical structure of temperature and wind under different future climate scenarios, including free-run simulations and three Shared Socioeconomic Pathways (SSP): SSP126, SSP370, and SSP585. These scenarios represent a range of potential greenhouse gas emissions trajectories, from low (SSP126) to high (SSP585) forcing conditions. The results confirm GAP’s stable vertical profiles across different climate regimes.

\begin{figure}[h]
\centering
\centerline{\includegraphics[width=0.8\linewidth]{suppli_fig/CESM_future_DJF_tem_vertical_history.jpg}}
\caption{GAP future projections (2070-2100) under different scenarios (free run, SSP126, SSP370 and SSP585). Resoults show DJF season zonal mean troposphere temperature.}\label{fig_CESM_t_vertical_DJF_future}
\end{figure}

Figures ~\ref{fig_CESM_t_vertical_DJF_future} and ~\ref{fig_CESM_t_vertical_JJA_future} present the vertical temperature structure across different scenarios. GAP demonstrates remarkable stability in maintaining physically consistent temperature profiles throughout the troposphere and stratosphere across all simulation periods. This stability is preserved even under high-forcing scenarios, where the model maintains appropriate lapse rates and thermal stratification patterns. The vertical structure in GAP simulations closely aligns with CESM2 constraints, indicating robust thermal representation across seasonal cycles and climate regimes.

\begin{figure}[h]
\centering
\centerline{\includegraphics[width=0.8\linewidth]{suppli_fig/CESM_future_JJA_u_vertical_history.jpg}}
\caption{GAP future projections (2070-2100) under different scenarios (free run, SSP126, SSP370 and SSP585). Resoults show JJA season zonal mean wind temperature.}\label{fig_CESM_u_vertical_JJA_future}
\end{figure}

Figures ~\ref{fig_CESM_u_vertical_JJA_future} and ~\ref{fig_CESM_u_vertical_DJF_future} illustrate the vertical wind structure under various climate forcing scenarios. GAP exhibits exceptional stability in reproducing zonal wind patterns, maintaining coherent upper-level westerlies and lower-level easterlies across all scenarios. The model preserves the characteristic vertical wind shear profiles essential for dynamic stability, with consistent representation of jet streams and their seasonal migrations. This stability in wind field representation underscores GAP's reliability in maintaining dynamically balanced atmospheric circulation patterns regardless of the underlying forcing conditions.

\begin{figure}[h]
\centering
\centerline{\includegraphics[width=0.8\linewidth]{suppli_fig/CESM_future_DJF_u_vertical_history.jpg}}
\caption{GAP future projections (2070-2100) under different scenarios (free run, SSP126, SSP370 and SSP585). Resoults show DJF season zonal mean wind temperature.}\label{fig_CESM_u_vertical_DJF_future}
\end{figure}

\begin{figure}[h]
\centering
\centerline{\includegraphics[width=0.6\linewidth]{suppli_fig/CESM_precip_bias_suppli.jpg}}
\caption{Spatial distribution of precipitable water of model and observation (a-c) and spatial average precipitable water model minus observations (ERA5) differences (d-e) for the 1979–2014 period from CESM2 and GAP.}\label{fig_CESM_precip_bias}
\end{figure}

Accurate simulation of precipitable water is critical for understanding the hydrological cycle and large-scale atmospheric dynamics. Figure~\ref{fig_CESM_precip_bias} highlights how GAP corrects systematic precipitable water biases, particularly in tropical and mid-latitude regions, where uncertainties in convection and moisture transport often degrade climate model accuracy. By leveraging generative modeling, GAP ensures that the simulated moisture distribution aligns closely with historical reanalysis data.

\clearpage

We observe interesting extreme events and key climate variability across different scenarios. we examine GAP's performance in capturing tropical cyclone trajectories (extreme events), Arctiv Oscillation (AO) and El Niño-Southern Oscillation (ENSO) variability under different climate scenarios, including free-run simulations and SSP126, SSP370, and SSP585 pathways. These tests assess whether GAP can faithfully reproduce historical climate patterns and extrapolate variability under future conditions.

Tropical cyclones are among the most extreme weather events, and their frequency, intensity, and tracks are expected to change with global warming and shifting atmospheric circulation. SI Fig. ~\ref{fig_CESM_tc_track1} presents ensemble simulations of tropical cyclone tracks across different climate scenarios. GAP successfully captures the observed spatial distribution of tropical cyclones, including their formation regions, movement patterns, and landfall probabilities, when compared with historical reanalysis.Under higher-emission scenarios (SSP370 and SSP585), GAP simulates increased cyclone intensity, consistent with established climate projections.

\begin{figure}[h]
\centering
\centerline{\includegraphics[width=0.8\linewidth]{suppli_fig/CESM_TC_track_suppli1.jpg}}
\caption{Tropical cyclone tracks for history (1850-2014) and future scenarios (free run and SSP126, 2015-2100). Four ensemble members are presented and the tracks are coloured in durations.}\label{fig_CESM_tc_track1}
\end{figure}

\begin{figure}[h]
\centering
\centerline{\includegraphics[width=0.55\linewidth]{suppli_fig/CESM_TC_track_suppli2.jpg}}
\caption{Tropical cyclone tracks for future scenario (SSP370 and SSP585, 2015-2100). Four ensemble members are presented and the tracks are coloured in durations.}\label{fig_CESM_tc_track2}
\end{figure}

The Arctic Oscillation (AO) is a key mode of atmospheric variability in the Northern Hemisphere, influencing mid-latitude weather patterns by modulating the strength of the polar vortex and associated westerly winds. Figure~\ref{fig_CESM_AO_suppli} presents the spatial patterns of AO variability simulated by GAP across different climate scenarios. In all scenarios, GAP successfully captures the characteristic AO dipole structure, with positive anomalies over the Arctic and negative anomalies over the mid-latitudes, consistent with observed AO patterns. However, notable differences emerge under future warming scenarios. In SSP370 and SSP585, GAP simulates an intensification of the AO pattern, with stronger positive anomalies in the high latitudes and more pronounced negative anomalies over the North Atlantic and Eurasia. This suggests a potential strengthening of the polar vortex and enhanced mid-latitude circulation changes under higher greenhouse gas forcing.

ENSO is a dominant mode of interannual climate variability, driving global-scale temperature and precipitation anomalies. The Southern Oscillation Index (SOI) serves as a key metric for ENSO variability, reflecting the pressure difference between the western and eastern Pacific. Figure~\ref{fig_CESM_SOI} shows that GAP, when constrained by SST-driven near-surface temperature (T2m), accurately reproduces historical SOI patterns, capturing both the frequency and amplitude of El Niño and La Niña events. In future projections, GAP preserves ENSO-like variability across SSP126, SSP370, and SSP585, with notable shifts in intensity and frequency under stronger warming scenarios. In SSP585, for example, ENSO events become more pronounced, aligning with projections of increased variability due to enhanced air-sea coupling.

\begin{figure}[h]
\centering
\centerline{\includegraphics[width=0.5\linewidth]{suppli_fig/fig_CESM_AO_suppli.jpg}}
\caption{Arctic Oscillation (AO) for future scenario (free run, SSP126, SSP370 and SSP585, 2060-2100). Positive and negative phases are coloured in blue and red respectively.}\label{fig_CESM_AO_suppli}
\end{figure}

\begin{figure}[h]
\centering
\centerline{\includegraphics[width=0.9\linewidth]{suppli_fig/CESM_soi_signals.pdf}}
\caption{Southern Oscillation Index (SOI) for future scenario (free run, SSP126, SSP370 and SSP585, 2060-2100). Positive and negative phases are coloured in blue and red respectively.}\label{fig_CESM_SOI}
\end{figure}

Figure~\ref{fig_CESM_tem_land} presents the temporal evolution of global mean land surface temperature anomalies across different climate scenarios. While GAP effectively captures the overall warming pattern, it exhibits a notable warm bias of approximately 0.5°C compared to CESM2 reference simulations. This systematic bias remains relatively consistent across both historical and future periods, suggesting structural differences in how GAP represents land surface processes. One possible reason for this bias is that CESM2 itself has systematic deviations from ERA5 reanalysis data, meaning that GAP, trained on CESM2 outputs, may have inherited this discrepancy. Despite this offset, the model successfully reproduces the relative warming magnitudes between different emission scenarios, maintaining the expected hierarchy of temperature responses.

\begin{figure}[h]
\centering
\centerline{\includegraphics[width=1\linewidth]{suppli_fig/CESM2_t2m_seris_land.pdf}}
\caption{Time series of the global mean surface air temperature over land for CESM2 with different senarios (solid coloured line) and GAP ensembles (shaded coloured area for model spread) with different senarios.}\label{fig_CESM_tem_land}
\end{figure}

The global mean temperature anomaly at 500 hPa (Fig.~\ref{fig_CESM_tem_seris_500hpa}) reflects the overall temperature change trend, indicating that GAP maintains physical consistency across different time scales. However, compared to CESM2, GAP fails to fully capture the amplitude of temperature variations, particularly under future warming scenarios, where its response appears more conservative. This limitation may be related to the model’s generalization capability—temperature changes at higher atmospheric levels are influenced by complex dynamical processes and radiative balance, which may not be fully captured by GAP’s statistical framework. Additionally, constraints in training data and the probabilistic modeling approach may contribute to an underestimation of extreme temperature variations.

\begin{figure}[h]
\centering
\centerline{\includegraphics[width=1\linewidth]{suppli_fig/CESM2_tem_seris_500hpa.pdf}}
\caption{Time series of the global-mean air temperature at 500 hpa for CESM2 with different senarios (solid coloured line) and GAP ensembles (shaded coloured area for model spread) with different senarios.}\label{fig_CESM_tem_seris_500hpa}
\end{figure}

Unlike traditional machine learning models, which often struggle with stability or unrealistic trends under high-emission scenarios, GAP maintains physically plausible atmospheric structures across multiple timescales. However, its potential limitations in generalization remain, as it may not fully capture the strength of emerging trends, particularly under strong warming scenarios. Despite some temperature biases, GAP demonstrates promise for long-term climate projections. Its ability to preserve dynamical coherence while effectively simulating future changes in atmospheric circulation, energy balance, and climate variability makes it a possible tool for studying climate evolution under different anthropogenic forcing conditions. This capability positions GAP as a potential framework for probabilistic climate risk assessment and long-term climate projections, offering new possibilities for exploring extreme events and large-scale climate oscillations.

\clearpage

\section{Supplementary visualization}
In this section we show supplementary cases and visualization of GAP, including unsupervised generation, assimilation and prediction across all time scales.

\subsection{Unsupervised generation}

SI Fig~\ref{fig_random_generation} presents a comparison between a meteorological field randomly generated using GAP and a corresponding field randomly selected from the ERA5 dataset. This comparison includes geopotential height, specific humidity, temperature, and the u and v components of wind at 500 hPa. Visually, the two fields exhibit strikingly similar patterns, with the generated field capturing physically plausible atmospheric circulation structures that align closely with those observed in the ERA5 dataset.

\begin{figure}[h]
\centering
\centerline{\includegraphics[width=0.8\linewidth]{suppli_fig/Generation_random.jpg}}
\caption{Comparison between GAP random generation and randomly sampled ERA5. Spatial fields at the 500 hPa pressure level are displayed: geopotential height (first row), specific humidity (second row), temperature (third row), u-component of wind (fourth row), and v-component of wind (fifth row). The third column presents the vertical profiles of these variables.)}\label{fig_random_generation}
\end{figure}

The geopotential height field generated by GAP successfully reproduces large-scale wave patterns and gradients, including prominent ridges and troughs that characterize synoptic-scale atmospheric dynamics. These features indicate that GAP effectively captures the spatial distribution and variations in pressure-related phenomena, which are critical for representing atmospheric circulation.

For specific humidity, the generated field closely matches the ERA5 dataset in both spatial distribution and intensity, particularly in regions dominated by strong moisture gradients, such as the Intertropical Convergence Zone (ITCZ) and mid-latitude storm tracks. This alignment reflects GAP's ability to accurately simulate hydrological processes and water vapor transport within the atmosphere, which are essential for understanding precipitation patterns and atmospheric moisture dynamics.

The temperature field generated by GAP maintains key climatological features, including the latitudinal temperature gradients and thermal contrasts between land and ocean surfaces. These patterns are essential for atmospheric stability and energy transfer. The similarity between the generated and ERA5 fields underscores GAP's capability to preserve realistic temperature structures, including those influenced by seasonal and regional variability.

The u and v components of wind fields produced by GAP also align well with ERA5, replicating the characteristic structures of mid-latitude jet streams, subtropical easterlies, and other wind systems. The accurate reproduction of these features highlights GAP's robustness in modeling the dynamic aspects of atmospheric circulation, ensuring that both zonal and meridional flows are consistent with observed patterns.

In addition to these visual comparisons, the mean field profiles across different altitudes demonstrate a high degree of consistency between the GAP-generated fields and ERA5 data. This agreement validates GAP's accuracy in representing the vertical distribution of atmospheric variables, further emphasizing its ability to generate realistic meteorological states. These results collectively highlight GAP's reliability and potential for generating physically consistent atmospheric fields suitable for research and operational applications.

\subsection{Ensemble assimilation}
Here, we present the ensemble assimilation results generated by GAP using operational meteorological observations. The assimilation experiments evaluate GAP's capability to generate diverse and physically consistent atmospheric fields for temperature, geopotential height, humidity, and wind, while effectively reducing forecast errors and ensemble spread through the assimilation process.

Figures~\ref{fig_obs_DA_t850}--\ref{fig_obs_DA_ws500} illustrate the assimilation results for key atmospheric variables. Specifically, Fig.~\ref{fig_obs_DA_t850} shows the temperature field at 850 hPa, Fig.~\ref{fig_obs_DA_q850} presents the specific humidity at 850 hPa, Fig.~\ref{fig_obs_DA_z500} depicts the geopotential height at 500 hPa, and Fig.~\ref{fig_obs_DA_ws500} displays the wind speed at 500 hPa. These results highlight GAP's ability to assimilate operational observations to generate realistic and diverse ensemble fields, capturing intricate spatial patterns across different meteorological variables.

\begin{figure}[h]
\centering
\centerline{\includegraphics[width=\linewidth]{suppli_fig/GAP_OBS_ens_z_suppli.jpg}}
\caption{An ensemble assimilation case generated from operational observations. The geopotential height at the 500 hPa pressure level is presented. The first row displays ERA5, IFS HERS analysis, and the GAP ensemble mean, while the subsequent rows depict the 50 ensemble members.}\label{fig_obs_DA_z500}
\end{figure}

\begin{figure}[h]
\centering
\centerline{\includegraphics[width=\linewidth]{suppli_fig/GAP_OBS_ens_q850_suppli.jpg}}
\caption{An ensemble assimilation case generated from operational observations. The specific humidity at the 500 hPa pressure level is presented. The first row displays ERA5, IFS HERS analysis, and the GAP ensemble mean, while the subsequent rows depict the 50 ensemble members.}\label{fig_obs_DA_q850}
\end{figure}

\begin{figure}[h]
\centering
\centerline{\includegraphics[width=\linewidth]{suppli_fig/GAP_OBS_ens_t2m_suppli.jpg}}
\caption{An ensemble assimilation case generated from operational observations. 2m temperature is presented. The first row displays ERA5, IFS HERS analysis, and the GAP ensemble mean, while the subsequent rows depict the 50 ensemble members.}\label{fig_obs_DA_t850}
\end{figure}

\begin{figure}[h]
\centering
\centerline{\includegraphics[width=\linewidth]{suppli_fig/GAP_OBS_ens_ws500_suppli.jpg}}
\caption{An ensemble assimilation case generated from operational observations. The wind speed at the 500 hPa pressure level is presented. The first row displays ERA5, IFS HERS analysis, and the GAP ensemble mean, while the subsequent rows depict the 50 ensemble members.}\label{fig_obs_DA_ws500}
\end{figure}

The temperature field (Fig.~\ref{fig_obs_DA_t850}) shows that GAP effectively reproduces large-scale thermal gradients and localized variations in temperature, including features associated with synoptic-scale weather systems. Similarly, the specific humidity field (Fig.~\ref{fig_obs_DA_q850}) reflects a strong alignment with moisture patterns, particularly in regions influenced by tropical convergence zones and mid-latitude cyclonic systems. 

The geopotential height assimilation results (Fig.~\ref{fig_obs_DA_z500}) demonstrate GAP's capacity to resolve planetary-scale wave structures and localized perturbations, capturing essential features of atmospheric circulation. Meanwhile, the wind speed field (Fig.~\ref{fig_obs_DA_ws500}) effectively replicates jet stream intensities, wind shear, and regional wind systems, indicating GAP's robustness in dynamic process simulation.

\clearpage

\subsection{Tropical cyclone tracks}\label{Tropical_cyclone_tracks}

SI Figs.~\ref{fig_TC_INFA_TRACK_ens}, \ref{fig_TC_DOKSURI_TRACK_ens}, and \ref{fig_TC_MAVAR_TRACK_ens} highlight how GAP ensemble forecasts can be applied to critical downstream applications, such as predicting the trajectories of tropical cyclones. We run a super ensemble experiments of 1000 ensembles for this 3 cases. These figures illustrate the predicted tracks for three significant typhoons: INFA, DOKSURI, and MAVAR. Each case demonstrates GAP's ability to represent both the uncertainty and evolving predictability of tropical cyclone paths over different forecast lead times.

\begin{figure}[h]
\centering
\centerline{\includegraphics[width=0.6\linewidth]{suppli_fig/TC_INFA_TRACK.jpg}}
\caption{The trajectory of Typhoon In-fa based on ERA5 (in red) and the ensemble of tropical cyclone trajectories from GAP (in grey) up to a validity time before the cyclone made rainfall in China. GAP forecasts are shown at lead time of 7 days.}\label{fig_TC_INFA_TRACK_ens}
\end{figure}

For Typhoon INFA, initialized seven days prior to its heavy rainfall in China, GAP’s ensemble forecasts capture a wide range of possible trajectories. The ensemble spread reflects the inherent uncertainty at longer lead times, highlighting potential variations in the storm’s path and landfall location. As the lead time decreases, the ensemble spread narrows, indicating increasing confidence in the predicted trajectory. By three days before landfall, GAP’s ensemble forecasts converge on a much tighter cluster of paths, accurately pinpointing the timing and location of landfall. This progression underscores GAP’s capability to dynamically adapt its forecasts as new observations are assimilated, providing reliable predictions even in complex meteorological scenarios.

\begin{figure}[h]
\centering
\centerline{\includegraphics[width=0.7\linewidth]{suppli_fig/TC_DOKSURI_TRACK.jpg}}
\caption{The trajectory of Typhoon Doksuri based on ERA5 (in red) and the ensemble of tropical cyclone trajectories from GAP (in grey) up to a validity time before the cyclone made rainfall in China. GAP forecasts are shown at lead time of 7 days.}\label{fig_TC_DOKSURI_TRACK_ens}
\end{figure}

Typhoon DOKSURI posed a different challenge due to its rapid intensification and curved trajectory over the western Pacific Ocean. GAP’s ensemble forecasts successfully captured the storm’s initial westward motion and subsequent sharp turn towards the northwest. At longer lead times, the ensemble spread reflects significant uncertainty about the timing and sharpness of this turn, which are critical factors in determining the cyclone’s impact on coastal regions. As the forecast window shortens, GAP’s predictions become increasingly aligned with the observed trajectory, providing accurate estimates of the cyclone’s landfall location and intensity. This case highlights GAP’s ability to handle the complex dynamics of rapidly evolving storms, where small changes in initial conditions can lead to significant differences in outcomes.

\begin{figure}[h]
\centering
\centerline{\includegraphics[width=0.7\linewidth]{suppli_fig/TC_MAVAR_TRACK.jpg}}
\caption{The trajectory of Typhoon Mavar based on ERA5 (in red) and the ensemble of tropical cyclone trajectories from GAP (in grey) up to a validity time before the cyclone made rainfall in Japan. GAP forecasts are shown at lead time of 15 days.}\label{fig_TC_MAVAR_TRACK_ens}
\end{figure}

For Typhoon MAVAR, GAP’s ensemble forecasts illustrate its skill in tracking cyclones over extended periods. MAVAR exhibited a relatively straightforward west-northwest trajectory, making it a valuable case for evaluating GAP’s performance in scenarios with lower intrinsic uncertainty. Even at seven days lead time, GAP’s ensemble spread remained relatively narrow, reflecting high confidence in the cyclone’s path. By the time MAVAR approached landfall, the ensemble forecasts provided precise estimates of the timing, location, and intensity of its impact. This case demonstrates GAP’s strength in maintaining forecast accuracy and consistency for cyclones with more predictable behavior.

The results from these three cases demonstrate GAP’s robust performance in tropical cyclone forecasting, particularly in representing the uncertainty and evolution of cyclone trajectories. The ensemble approach enables GAP to provide probabilistic predictions that account for a range of possible outcomes, offering valuable information for risk assessment and decision-making. The narrowing of ensemble spread as lead times shorten reflects the model’s ability to incorporate new data, reducing uncertainty and increasing forecast reliability.

These capabilities are critical for operational applications, such as disaster preparedness and resource allocation. By providing both the most likely outcomes and the associated uncertainty, GAP empowers decision-makers to make informed choices in the face of extreme weather events. The demonstrated accuracy and adaptability of GAP in these three typhoon cases establish it as a powerful tool for tropical cyclone prediction and related downstream applications.

%\clearpage

\subsection{Seasonal cycle}\label{SI_seasonalcycle}

We conducted a 1,050-year simulation without prescribed external forcing, referred to as a free-run experiment. This experiment was initialized in 1980 and extends through the year 3030. The full global mean 2m temperature time series is shown in SI Fig. \ref{fig_global_2m_temperature_1000yr_case}.

\begin{figure}[h]
\centering
\centerline{\includegraphics[width=0.9\linewidth]{suppli_fig/global_2m_temperature_1000yr_suppli.jpg}}
\caption{ Global mean surface air temperature for a 1050-year free run simulation of GAP. Full year intervals (1980-3030) are selected showing a very good reproduction of the seasonal cycle.}\label{fig_global_2m_temperature_1000yr_case}
\end{figure}

The results demonstrate that GAP excels in maintaining stable and consistent modeling, even under free-run conditions without external constraints. Over the course of 1,050 years, GAP not only preserves a robust seasonal cycle but also accurately captures long-term variability. This highlights its ability to model inherent atmospheric dynamics over extended timescales without deviating from physical plausibility.

While some outliers are observed in the time series, GAP effectively reverts these deviations back to a reasonable trajectory, thanks to its strong climatological priors. This capability ensures that the simulation remains physically consistent and avoids the accumulation of errors that could otherwise destabilize long-term projections.

The stable performance of GAP in this extended free-run scenario underscores its reliability and potential for long-term climate simulations. Such experiments are crucial for understanding intrinsic variability in the Earth system and evaluating the performance of models in scenarios where external forcing is not applied. GAP’s ability to maintain a realistic climatology and seasonal cycle over millennia further reinforces its utility for climate research and long-term predictive modeling.

To evaluate GAP's ability to emulate seasonal cycles across various spatial scales, we conducted a one-year free-run ensemble experiment (SI Fig. \ref{fig_CFS_t2m_case}). This experiment examined temperature variations over four regions: the globe, Eurasia, China, and Beijing. The results demonstrate that all ensemble members effectively replicate the seasonal cycle at each spatial scale, showcasing GAP's robustness in capturing both regional and global temperature patterns.

\begin{figure}[h]
\centering
\centerline{\includegraphics[width=0.9\linewidth]{suppli_fig/Suppli_CFS_t2m.pdf}}
\caption{Global mean, regional mean and grid based surface air temperature for a one-year ensemble prediction of GAP. It shows a very good reproduction of the seasonal cycle across all spatial scale.}\label{fig_CFS_t2m_case}
\end{figure}

Additionally, the analysis includes temperature anomalies, providing insights into GAP's capacity to simulate and predict deviations from the climatological mean. The ensemble results reveal that GAP can successfully capture variations in temperature anomalies, highlighting its sensitivity to natural variability and its ability to represent smaller-scale fluctuations.

This performance is particularly significant for applications in seasonal prediction. The ability of GAP's ensemble to maintain consistency in seasonal cycles and accurately reflect temperature anomalies suggests its strong potential as a tool for seasonal forecasting. These findings serve as compelling evidence of GAP's utility for predicting seasonal variations across different spatial scales, reinforcing its applicability in both operational and research-oriented climate studies.

%\begin{figure}[h]
%\centering
%\centerline{\includegraphics[width=\linewidth]{suppli_fig/TC_climatology.jpg}}
%\caption{Tropical cyclone climatology}\label{fig_tropical_cyclone_climatology_case}
%\end{figure}

%\begin{figure}[h]
%\centering
%\centerline{\includegraphics[width=\linewidth]{suppli_fig/Block_climatology.jpg}}
%\caption{Blocking climatology}\label{fig_block_climatology_case}
%\end{figure}

%\begin{figure}[h]
%\centering
%\centerline{\includegraphics[width=\linewidth]{suppli_fig/AMIP_soi_signals.jpg}}
%\caption{SOI time series}\label{fig_SOI_case}
%\end{figure}

\clearpage

\putbib[sn-bibliography-suppli]
\end{bibunit}

%\end{document}
